# Supplementary material for: Varieties of Nodal surfaces, coding theory and Discriminants of cubic hypersurfaces. Part 1: Generalities and nodal K3 surfaces. Part 2: Cubic Hypersurfaces, associated discriminants. Part 3: Nodal quintics. Part 4: Nodal sextics
Source: arXiv:2206.05492 ancillary file (2025-06-05)
Supplement: Supplementary file 1 [file TexifiedScripts_NodalSeveri.pdf]

# SCRIPTS FOR “VARIETIES OF NODAL SURFACES, CODING THEORY AND DISCRIMINANTS OF CUBIC HYPERSURFACES”

YONGHWA CHO, STEPHEN COUGHLAN, DAVIDE FRAPPORTI, AND MICHAEL KIERMAIER

ABSTRACT. This article is to deliver a better access to the scripts for the article *Varieties of nodal surfaces, coding theory and discriminants of cubic hypersurfaces* ([arXiv:2206.05492](https://arxiv.org/abs/2206.05492)). We provide the colored T<sub>E</sub>Xified version as well as the original scripts which are enclosed in the same arXiv submission.

## CONTENTS

|                                                               |    |
|---------------------------------------------------------------|----|
| 1. Overall guide                                              | 1  |
| 2. Mathematica & Macaulay2 scripts by Yonghwa Cho             | 1  |
| 2.1. Structure of the (extended) code                         | 1  |
| 2.2. Explicit determinantal equation                          | 9  |
| 2.3. General sextic with 65 nodes                             | 17 |
| 3. Magma scripts by Michael Kiermaier                         | 22 |
| 4. Magma scripts by Stephen Coughlan & Davide Frapporti       | 31 |
| 4.1. Studying lines through nodes on the Barth sextic surface | 31 |
| 4.2. Finding 2-planes in the Goryunov–Kalker cubic            | 37 |
| References                                                    | 40 |

## 1. OVERALL GUIDE

In this article we provide the scripts supporting [2]. These scripts are written over a number of computer algebra systems, namely, Mathematica, MAGMA, and Macaulay2. For this reason, we provide a single T<sub>E</sub>Xified version of the scripts for the reader’s convenience. The original script files are also enclosed in this arXiv submission. The following is the list of script files corresponding to each section.

§2: `ExtendedCode.nb` (Mathematica), `ExtendedCode.m2` and `ExtendedCode_Setup.m2` (Macaulay2).  
 §3: `BarthCode.m`  
 §4: `BarthNodeLines.m` (§4.1), and `GK2Planes.m` (§4.2).

## 2. MATHEMATICA & MACAULAY2 SCRIPTS BY YONGHWA CHO

### 2.1. Structure of the (extended) code.

Following series of scripts (Mathematica 1–10) are about basic structure of the (extended) code of Barth sextic surface, including the implementation of the  $\mathfrak{A}_5$ -representation. See *Part 4*, §3 in [2] for the usage of these scripts.

---

#### MATHEMATICA 1. $\mathfrak{A}_5$ -representation of codes

---

```

1  (* Build up A_5-representation *)
2
3  (* AppendBlock: Insert block_ into matrix_, fitting block[[1,1]] with matrix[[i,j]] *)
4  AppendBlock[i_, j_, matrix_, block_] := Module[{k, l, ret = matrix},

```

```

5     For[k = 1, k <= Dimensions[block][[1]], k++,
6     For[l = 1, l <= Dimensions[block][[2]], l++,
7         ret[[k + i - 1, l + j - 1]] =
8             matrix[[k + i - 1, l + j - 1]] + block[[k, l]];
9     ];
10 ];
11 ret
12 ];
13
14 (* BlockDiagonal : unify the given (rectangular) matrices into one block diagonal matrix *)
15 BlockDiagonal[matrix_] := Module[{k, s = 1, ret, size = {0, 0}},
16     For[k = 1, k <= Length[matrix], k++,
17         size = size + Dimensions[matrix[[k]]];
18     ];
19     ret = Normal[SparseArray[{i_, j_} -> 0, {size[[1]], size[[2]]}]];
20     size = {1, 1};
21     For[k = 1, k <= Length[matrix], k++,
22         ret = AppendBlock[size[[1]], size[[2]], ret, matrix[[k]];
23         size = size + Dimensions[matrix[[k]]];
24     ];
25     ret
26 ];
27
28 (* Permutation Matrices *)
29
30 H = AbelianGroup[{2, 2, 2}]; (* H := (Z/2Z)^3 *)
31 HList = GroupElements[H];
32 HMatrix = {};
33 HGen = {};
34
35 (* G := A_5 *)
36 σG = Cycles[{{1, 2, 3}}]; τG = Cycles[{{1, 4}, {2, 5}}]; (* Pick two generators of A_5 *)
37 G = PermutationGroup[ {σG, τG}];
38 GList = GroupElements[G];
39 GMatrix = {};
40 GGen = {};
41 T = {{0, 1}, {1, 0}};
42
43 (* Construct the matrix of (1,0,0) ∈ H *)
44 hA = BlockDiagonal[{T, T, T, T, T, IdentityMatrix[3]}];
45 B = Normal[SparseArray[{i_, j_} -> 0, {8, 8}]];
46 B = AppendBlock[1, 1, B, T];
47 B = AppendBlock[3, 7, B, T];
48 B = AppendBlock[5, 5, B, T];
49 B = AppendBlock[7, 3, B, T];
50 hB = BlockDiagonal[{B, B, B, T, IdentityMatrix[4]}];
51 hC = BlockDiagonal[{B, IdentityMatrix[4], T, T, T, T}];
52 HGen = Append[HGen, BlockDiagonal[{{1}}, hA, hB, hC]]; (* HGen[[1]] = h_100 *)
53 MatrixForm[HGen[[1]]];
54
55
56 (* Construct the matrix of (0,1,0) ∈ H *)
57 U = Normal[SparseArray[{i_, j_} -> 0, {4, 4}]];
58 U = AppendBlock[1, 3, U, IdentityMatrix[2]];
59 U = AppendBlock[3, 1, U, IdentityMatrix[2]];
60 hA = BlockDiagonal[{U, U, U, IdentityMatrix[3]}];
61 B = Normal[ SparseArray[ {{1, 3}, {2, 8}, {3, 1}, {4, 6}, {5, 7}, {6, 4}, {7, 5}, {8, 2}} -> 1,
62     {8, 8}} ];
63 hB = BlockDiagonal[{B, B, B, IdentityMatrix[2], T, IdentityMatrix[2]}];
64 TT = Normal[SparseArray[{i_, j_} -> 0, {4, 4}]];
65 TT = AppendBlock[1, 3, TT, T];

```

```

65 TT = AppendBlock[3, 1, TT, T];
66 hC = BlockDiagonal[{B, T, T, IdentityMatrix[4], TT}];
67 HGen = Append[HGen, BlockDiagonal[{{1}}, hA, hB, hC]]; (* HGen[[2]] = h_010 *)
68
69 (* Construct the matrix of (0,0,1) ∈ H *)
70 hA = BlockDiagonal[{TT, TT, TT, IdentityMatrix[3]}];
71 B = Normal[SparseArray[{{1, 4}, {2, 7}, {3, 6}, {4, 1}, {5, 8}, {6, 3}, {7, 2}, {8, 5}} -> 1,
    {8, 8}]];
72 hB = BlockDiagonal[{B, B, B, IdentityMatrix[4], T}];
73 hC = BlockDiagonal[{B, TT, TT, IdentityMatrix[4]}];
74 HGen = Append[HGen, BlockDiagonal[{{1}}, hA, hB, hC]]; (* HGen[[2]] = Subscript[h, 010] *)
75 MatrixForm[HGen[[3]]];
76
77 (* Construct "HMatrix", the list consisting of elements in the image of  $\rho_H : H \rightarrow GL(F_2^{66})$ 
78 The rule is : HMatrix[[j]] =  $\rho_H$  ( HList[[j]] ) *)
79
80 (* GroupHom : Given image of generators, compute the set-theoretic image of
81 the group homomorphism G -> GL(F_2^{66}) *)
82 GroupHom[Group_, GenMatrix_] :=
83 Module[{Wordlist, GList, T, i, j, ret = {}},
84 GList = GroupElements[Group];
85 For[i = 1, i <= Length[GList], i++,
86 T = IdentityMatrix[66];
87 Wordlist = GroupElementToWord[Group, GList[[i]]];
88 For[j = 1, j <= Length[Wordlist], j++,
89 If[Wordlist[[j]] > 0, T = GenMatrix[[Wordlist[[j]]]].T];
90 If[Wordlist[[j]] < 0,
91 T = Inverse[GenMatrix[{-Wordlist[[j]]}]].T];
92 ];
93 ret = Append[ret, T];
94 ];
95 ret
96 ];
97 HMatrix = GroupHom[H, HGen];
98
99 (* Do the same job for G = A_5 *)
100 (* Construct the matrix associated to the permutation ( i -> Perm[[i]] ) *)
101 PermutationMatrix[Perm_] := Module[{TempList = {}, g},
102 For[i = 1, i <= Length[Perm], i++,
103 TempList = Append[TempList, {Perm[[i]], i}];
104 ];
105 Normal[SparseArray[TempList -> 1, {Length[Perm], Length[Perm]}]]
106 ];
107  $\sigma A$  = PermutationMatrix[{10, 15, 5, 2, 12, 8, 1, 14, 13, 7, 9, 3, 11, 6, 4}];
108  $\sigma B$  = PermutationMatrix[{22, 30, 9, 6, 18, 29, 13, 2, 20, 12, 1, 28, 24, 16, 5, 27, 25, 15, 17,
    3, 26, 11, 21, 7, 19, 23, 14, 10, 4, 8}];
109  $\sigma C$  = PermutationMatrix[{16, 12, 1, 20, 14, 10, 5, 18, 4, 17, 8, 19, 13, 7, 15, 3, 6, 11, 2,
    9}];
110
111 GGen = Append[GGen, BlockDiagonal[{{1}},  $\sigma A$ ,  $\sigma B$ ,  $\sigma C$ ]]; (* GGen[[1]] =  $\rho_G(\sigma)$  *)
112
113  $\tau A$  = PermutationMatrix[{11, 2, 14, 7, 13, 10, 4, 8, 9, 6, 1, 15, 5, 3, 12}];
114  $\tau B$  = PermutationMatrix[{19, 6, 27, 11, 23, 2, 28, 15, 25, 22, 4, 16, 26, 18, 8, 12, 17, 14, 1,
    29, 21, 10, 5, 30, 9, 13, 3, 7, 20, 24}];
115  $\tau C$  = PermutationMatrix[{13, 6, 17, 10, 15, 2, 19, 12, 16, 4, 14, 8, 1, 11, 5, 9, 3, 20, 7,
    18}];
116
117 GGen = Append[GGen, BlockDiagonal[{{1}},  $\tau A$ ,  $\tau B$ ,  $\tau C$ ]]; (* GGen[[2]] =  $\rho_G(\tau)$  *)
118 GMatrix = GroupHom[G, GGen];
119
120 (* Extend the Code by action of given group representation *)

```



---

MATHEMATICA 3. Finding  $G$ -orbits

---

```

1  SetAttributes[GOrbit, HoldAll];
2  (* Given a set codewords_ and G-representation, find the G-orbit *)
3  GOrbit[codewords_, GMatrix_, GroupSpanningElement_] :=
4  Module[{i, j, ilen = Length[codewords], jlen = Length[GMatrix], tmp, ret},
5    ret = List[];
6    For[i = 1, i <= ilen, i++,
7      For[j = 1, j <= jlen, j++,
8        (* To store the data more concisely, use decimal expansion of  $\text{ret} \in \{F_2^{66}\}$  *)
9        tmp = FromDigits[GMatrix[[j]].codewords[[i]], 2];
10       If[Count[ret, tmp] == 0,
11         AppendTo[ret, tmp];
12         AppendTo[GroupSpanningElement, {i, GList[[j]]}];
13         (* Record which codeword and which group element generate the word *)
14       ];
15     ];
16   ];
17   ret
18 ];
19
20 (* Finding the set of weight 16 half even sets *)
21 GSpanElements = {};
22 HSpanElements = {};
23 W16SpanElements = {};
24 GSet = GOrbit[{v4}, GMatrix, GSpanElements]; (* A5-orbit of v4 -> 20 codewords *)
25 HSet = GOrbit[{v1, v2, v3}, HMatrix, HSpanElements];
26 (* H-orbit of {v1,v2,v3} -> 6 codewords *)
27 W16Set = Join[GSet, HSet]
28 (* results the (duplicate-free) list of length 26: the 15-half even sets *)

```

---



---

MATHEMATICA 4. Weight enumeration

---

```

1  (* Find the codeword corresponding to the binary expansion of the input "num"
2  eg: Codeword[Code, 16+8+1] returns sum Code[[5]]+Code[[4]]+Code[[1]] (Mod 2) *)
3  Codeword[Code_, subsets_] :=
4  Module[{i, ilen, binsubsets, listsubset, word},
5    binsubsets = IntegerDigits[subsets, 2];
6    listsubset =
7      Length[binsubsets] + 1 - Flatten[Position[binsubsets, 1]];
8    Mod[Total[Code[[listsubset]]], 2]
9  ];
10
11 (* Compute the weight enumerator of the given code *)
12 WeightEnumeration[Code_] :=
13 Module[{i, j, ilen, countlist, ibin, dim, v},
14   ilen = 2^Length[Code];
15   dim = Dimensions[Code][[2]];
16   countlist = Normal[SparseArray[i_ -> 0, dim]];
17   For[i = 1, i <= ilen - 1, i++,
18     v = Codeword[Code, i];
19     countlist[[Total[v]]] = countlist[[Total[v]]] + 1;
20   ];
21   For[i = 1, i <= dim, i++,

```

```

22     If[countlist[[i]] != 0 ,
23         Print["Number of nonzero codewords with weight ", i, " = ",
24             countlist[[i]]];
25     ];
26 ];
27 ];
28
29 (* weight enumerator of both strict and extended code *)
30
31 StrictCode = Take[GCode, {2, Length[GCode]}, {2, 66}];
32 WeightEnumeration[StrictCode] (* Weight enumerator of strict code *)
33 WeightEnumeration[GCode] (* Weight enumerator of extended code *)

```

---

## MATHEMATICA 5. $k$ -sums having fixed weight

---

```

1  (* For the counter of the nested loop *)
2  CountNext[Countlist_, Cap_] :=
3  Module[{ret, flg, i, ilen = Length[Countlist], valueatflg},
4      ret = Countlist;
5      If[Countlist[[ilen]] < Cap,
6          ret[[ilen]] = Countlist[[ilen]] + 1,
7          (* if the last term of Countlist acheives the maximum *)
8
9          flg = ilen;
10         For[i = 1, i <= ilen - 1, i++,
11             If[Countlist[[i]] < Cap + i - ilen,
12                 flg = i;
13             ];
14         ];
15         If[flg == ilen, ret[[1]] = Cap + 1,
16             valueatflg = Countlist[[flg]];
17         For[i = flg, i <= ilen, i++,
18             ret[[i]] = valueatflg + (i - flg + 1);
19         ];
20     ];
21 ];(*If ends*)
22 ret
23 ];
24
25 (* Construct the list of codewords which
26 (1) can be written as the sum of precisely k_ distinct elements in GSet_
27 (2) has weight = weight_ *)
28 kSpan[GSet_, k_, weight_] :=
29 Module[{tmpbin, tmp, ret, Glen = Length[GSet], looplist = {}, i},
30     ret = {};
31     For[i = 1, i <= k, i++,
32         AppendTo[looplist, i];
33     ];
34     While[looplist[[1]] <= Glen,
35         tmpbin = 0;
36         For[i = 1, i <= k, i++,
37             tmpbin = tmpbin + IntegerDigits[ GSet[[ looplist[[i]] ]], 2, 66] ;
38         ];
39         tmpbin = Mod[tmpbin, 2];

```

```

40     tmp = FromDigits[tmpbin, 2];
41     If[Total[tmpbin] == weight && Count[ret, tmp] == 0,
42       AppendTo[ret, tmp];
43     ];
44     looplist = CountNext[looplist, Glen];
45   ];
46   ret
47 ];
48
49   SpanGSet = kSpan[W16Set, 3, 32];
50   (* The list of half even sets of cardinality 31 that can be written as a sum of three
      half even sets of cardinality 15 *)

```

---

#### MATHEMATICA 6. The half even sets of cardinality 31 that admit $15 + 24$ decomposition

---

```

1  (* Find the even set of cardinality 24, which CANNOT be written as a sum of two plane sections
   *)
2  list2 = Block[{Print}, kSpan[W16Set, 2, 24]];
3  list4 = Block[{Print}, kSpan[W16Set, 4, 24]];
4  (* ProperEven24 := 65 even sets that are not written as sum of two planar sections *)
5  ProperEven24 = Complement[list4, list2];
6
7  (* Assertion: the remaining 390(=1690-1300) 31-half even sets are the sums of half-quadric and
   half-linear sections *)
8  ProperJoin = Join[ProperEven24, W16Set];
9  tmplist = Block[{Print}, kSpan[ProperJoin, 2, 32]];
10  (* There are two classes in this list.
   (1) half even sets of cardinality 31 with 15+24 decomposition
   (2) even sets of cardinality 32 with 24+24 decomposition *)
11
12
13
14  (* Exclude the case (2) *)
15  Proper31 = {};
16  For[i = 1, i <= Length[tmplist], i++,
17    If[tmplist[[i]] >= 2^65, (* count only half even sets *)
18      AppendTo[Proper31, tmplist[[i]]];
19    ];
20  ];
21  (* Proper31 has 390 elements, so the "Assertion" above is true *)

```

---

#### MATHEMATICA 7. Coordinates of the nodes in Barth's sextic

---

```

1   $\tau = (1 + \text{Sqrt}[5])/2;$ 
2   $\tau' = (1 - \text{Sqrt}[5])/2;$ 
3  NodeList = {
4    {0, 0, 0, 0}, (* A temporary elements to make the list coherent with the extended codes *)
5  (* 15 Nodes of Type A *)
6    {0, 1,  $\tau$ ,  $-\tau'$ }, {0, -1,  $\tau$ ,  $-\tau'$ }, {0, 1,  $-\tau$ ,  $-\tau'$ }, {0, 1,  $\tau$ ,  $\tau'$ },

```

```

7      {0, - $\tau'$ , 1,  $\tau$ }, {0,  $\tau'$ , 1,  $\tau$ }, {0, - $\tau'$ , -1,  $\tau$ }, {0, - $\tau'$ , 1, - $\tau$ },
8      {0,  $\tau$ , - $\tau'$ , 1}, {0, - $\tau$ , - $\tau'$ , 1}, {0,  $\tau$ ,  $\tau'$ , 1}, {0,  $\tau$ , - $\tau'$ , -1},
9      {0, 1, 0, 0}, {0, 0, 1, 0}, {0, 0, 0, 1},
10
11     (* 30 Nodes of Type B *)
12     {2, 1,  $\tau$ , - $\tau'$ }, {2, -1,  $\tau$ , - $\tau'$ }, {2, 1, - $\tau$ , - $\tau'$ }, {2, 1,  $\tau$ ,  $\tau'$ },
13     {2, -1, - $\tau$ ,  $\tau'$ }, {2, 1, - $\tau$ ,  $\tau'$ }, {2, -1,  $\tau$ ,  $\tau'$ }, {2, -1, - $\tau$ , - $\tau'$ },
14     {2, - $\tau'$ , 1,  $\tau$ }, {2,  $\tau'$ , 1,  $\tau$ }, {2, - $\tau'$ , -1,  $\tau$ }, {2, - $\tau'$ , 1, - $\tau$ },
15     {2,  $\tau'$ , -1, - $\tau$ }, {2, - $\tau'$ , -1, - $\tau$ }, {2,  $\tau'$ , 1, - $\tau$ }, {2,  $\tau'$ , -1,  $\tau$ },
16     {2,  $\tau$ , - $\tau'$ , 1}, {2, - $\tau$ , - $\tau'$ , 1}, {2,  $\tau$ ,  $\tau'$ , 1}, {2,  $\tau$ , - $\tau'$ , -1},
17     {2, - $\tau$ ,  $\tau'$ , -1}, {2,  $\tau$ ,  $\tau'$ , -1}, {2, - $\tau$ , - $\tau'$ , -1}, {2, - $\tau$ ,  $\tau'$ , 1},
18     {1, 1, 0, 0}, {1, -1, 0, 0}, {1, 0, 1, 0}, {1, 0, -1, 0}, {1, 0, 0, 1}, {1, 0, 0, -1},
19
20     (* 20 Nodes of Type C *)
21     {1, 1, 1, 1}, {1, -1, 1, 1}, {1, 1, -1, 1}, {1, 1, 1, -1},
22     {1, -1, -1, -1}, {1, 1, -1, -1}, {1, -1, 1, -1}, {1, -1, -1, 1},
23     {1, 0, - $\tau'$ ,  $\tau$ }, {1, 0,  $\tau'$ ,  $\tau$ }, {1, 0,  $\tau'$ , - $\tau$ }, {1, 0, - $\tau'$ , - $\tau$ },
24     {1,  $\tau$ , 0, - $\tau'$ }, {1, - $\tau$ , 0, - $\tau'$ }, {1, - $\tau$ , 0,  $\tau'$ }, {1,  $\tau$ , 0,  $\tau'$ },
25     {1, - $\tau'$ ,  $\tau$ , 0}, {1,  $\tau'$ ,  $\tau$ , 0}, {1,  $\tau'$ , - $\tau$ , 0}, {1, - $\tau'$ , - $\tau$ , 0}
26 };

```

---

## MATHEMATICA 8. On the generating sets of the code

---

```

1  decGenSet = ProperEven24; (* The set of even sets of cardinality 24 that does not admit 15+15
   decomposition. These correspond to  $S_3$ -spheres of the Doro-Hall graph *)
2  binGenSet=IntegerDigits[decGenSet, 2, 66];
3  SubCode=RowReduce[binGenSet, Modulus -> 2];
4  MatrixRank[SubCode] == 12
5  (* By setting decGenSet=W16Set, we get the matrix of rank 13, so the 26 half even sets of
   cardinality 15 generate the extended code *)

```

---

## MATHEMATICA 9. $k$ -decompositions

---

```

1
2  (* Find the sum of codewords *)
3  CodewordsSum[decCode_, sublist_] :=
4  Module[{ret, binCode, i, ilen = Length[sublist]},
5    binCode = IntegerDigits[decCode[[sublist]], 2, 66];
6    ret = Mod[Total[binCode], 2]
7    ];
8
9  (* Given a half even set, list the all possible decomposition into  $k_*$  (distinct) members of
   GSet_ *)
10 FindDecompositions[decCodeword_, GSet_,  $k_*$ ] :=
11 Module[{listCount, Glen = Length[GSet], tmpsum, globalFlg = False,
12   retlist = {}},
13   listCount = Array[# &, { $k_*$ };

```



```

14 While[listCount[[1]] <= Glen,
15   tmpsum = FromDigits[ CodewordsSum[GSet, listCount], 2];
16   If[tmpsum == decCodeword,
17     AppendTo[retlist, listCount];
18   ];
19   listCount = CountNext[listCount, Glen];
20 ];
21 retlist
22 ];

```

---

## MATHEMATICA 10. On Barth graph

---

```

1  (* Construct the adjacency matrix of Barth graph *)
2  F[{w_, x_, y_, z_}] := ( $\tau^2 x^2 - y^2$ ) ( $\tau^2 y^2 - z^2$ ) ( $\tau^2 z^2 - x^2$ ) - (2  $\tau + 1$ )/4 * w^2
   (  $x^2 + y^2 + z^2 - w^2$  )^2;
3  AdjMat = ConstantArray[0, {65, 65}];
4  For[i = 1, i <= 65, i++,
5    For[j = i + 1, j <= 65, j++,
6      (* Pick two nodes *)
7      P1 = NodeList[[i + 1]];
8      P2 = NodeList[[j + 1]];
9
10     (* Parametrize the line (t -> P1+t*P2) and find the intersection (except double t=0) with
       Barth sextic *)
11     intersections = Solve[Simplify[F[P1 + t*P2]/(t^2)] == 0, t];
12     intersections = DeleteDuplicates[intersections]; (* Then, remove the multiple roots *)
13     If[Length[intersections] == 2,
14       If[Simplify[t /. intersections[[1]]] != 0 && Simplify[t /. intersections[[2]]] != 0,
15         AdjMat[[i]][[j]] = 1;
16         AdjMat[[j]][[i]] = 1;
17       ];
18     ];
19   ];
20 ];
21
22 (* Is Barth graph locally Petersen? *)
23 BarthGraph = AdjacencyGraph[AdjMat]; (* Construct Barth graph using adjacency matrix *)
24 Petersen = GraphData["PetersenGraph"]; (* Load Petersen graph *)
25
26 (* For each vertex, find punctured neighborhoods and check whether they are isomorphic to
   Petersen graph *)
27 isLocallyPetersen = True;
28 For[v = 1, v <= 65, v++,
29   nbhdGraph = NeighborhoodGraph[BarthGraph, v];
30   isPetersen = Subgraph[nbhdGraph, Complement[VertexList[nbhdGraph], {v}]];
31   isLocallyPetersen = isLocallyPetersen && IsomorphicGraphQ[Petersen, isPetersen];
32 ];
33 isLocallyPetersen
34
35 (* 3-spheres are even sets of cardinality 24 that do not admit 15+15 decompositions *)
36 GraphDistanceMatrix[BarthGraph];
37 binThreeSpheres = Floor[%/3];
38 dec3Spheres = FromDigits[binThreeSpheres, 2];
39 Sort[dec3Spheres] == Sort[ProperEven24]

```

## 2.2. Explicit determinantal equation.

The following scripts (Mathematica 11 through Mathematica 17) are the computations of explicit determinantal presentations of Barth sextic surface following the method developed in [1]. The corresponding part is *Part 2, §4* in [2].

---

### MATHEMATICA 11. Finding equations passing through a set of nodes

---

```

1  (* Manipulation on Veronese coordinates *)
2  (* For the multidegree loops *)
3  CountNextMultiDegree[MultiDeg_] :=
4  Module[{ret = MultiDeg, totalDeg = Total[MultiDeg], LastNonzero, i,
5    len = Length[MultiDeg]},
6    For[i = len - 1, MultiDeg[[i]] == 0 && i >= 1, i--];
7    LastNonzero = i;
8    If[0 < LastNonzero && LastNonzero < len - 1,
9      ret[[LastNonzero]]--;
10     ret[[LastNonzero + 1]] = 1 + ret[[len]];
11     ret[[len]] = 0,
12     (*else*)
13     ret[[len - 1]]--;
14     ret[[len]]++;
15     ];
16    If[LastNonzero == 0, ret[[1]] = totalDeg + 1];
17    ret
18  ];
19
20  (* Translate a given linear coordinates into degree deg_ Veronese coordinates *)
21  GetVeroneseCoordinates[Coordinate_, deg_] :=
22  Module[{i, ret = {}, MultiDeg = {deg, 0, 0, 0},
23    EvaluatedVeroneseMonomial, multiplier},
24    While[MultiDeg[[1]] <= deg,
25      EvaluatedVeroneseMonomial = 1;
26      For[i = 1, i <= 4, i++,
27        If[Coordinate[[i]] == 0 && MultiDeg[[i]] == 0, (*Do nothing*),
28          EvaluatedVeroneseMonomial =
29            EvaluatedVeroneseMonomial*Coordinate[[i]]^MultiDeg[[i]];
30        ];
31      ];
32      AppendTo[ret, EvaluatedVeroneseMonomial];
33      MultiDeg = CountNextMultiDegree[MultiDeg];
34    ];
35    ret
36  ];
37  CodewordToVeroneseCoordinates[binCodeword_, deg_] :=
38  Module[{i, ret = {}},
39    For[i = 2, i <= 66, i++,
40      If[binCodeword[[i]] == 1,
41        AppendTo[ret, GetVeroneseCoordinates[NodeList[[i]], deg]];
42      ];
43    ];
44    ret
45  ];

```

```

46
47 ExtractEquations[binCodewords_, totalDeg_] :=
48   Module[{itemlen = Binomial[3 + totalDeg, 3],
49     len = Length[binCodewords], VeroneseCoordinates = {}, tmpList, i, j, v, Av},
50   For[i = 1, i <= len, i++,
51     tmpList = CodewordToVeroneseCoordinates[binCodewords[[i]], totalDeg];
52     For[j = 1, j <= Length[tmpList], j++,
53       If[Count[VeroneseCoordinates, tmpList[[j]]] == 0,
54         AppendTo[VeroneseCoordinates, tmpList[[j]]];
55         (* Collect the Veronese coordinates of the nodes in binCodewords_ *)
56       ];
57     ];
58   ];
59   VeroneseCoordinates = DeleteCases[RowReduce[VeroneseCoordinates], ConstantArray[0, itemlen]];
60   (* VeroneseCoordinates gives the linear system whose solutions are the coefficients of
61     the degree totalDeg_ polynomials passing through the nodes *)
62   v = GetVeroneseCoordinates[{w, x, y, z}, totalDeg];
63   Av = {};
64   For[i = 1, i <= itemlen, i++,
65     AppendTo[Av, Subscript[a, v[[i]]]];
66   ];
67   Print[MatrixForm[VeroneseCoordinates], "\t->\t",
68     MatrixForm[VeroneseCoordinates.Av]];
69   VeroneseCoordinates
70 ];
71
72 (* Translate the result of ExtractEquations into the equation form *)
73 MatrixToEquations[CoeffMatrix_, Coordinates_, deg_] :=
74   Module[{retPoly = 0, VeroneseCoordinates, i, ilen = Length[CoeffMatrix], j, jlen, jlen1,
75     depList, depDualList = {}, depPos, indepList = {},
76     indepListStr = "Independent variables are (Format: Subscript[a, ...]):\t"},
77   VeroneseCoordinates = GetVeroneseCoordinates[Coordinates, deg];
78   jlen = Length[VeroneseCoordinates];
79   depList = ConstantArray[0, {jlen}]; (* Mark 1 if the corresponding variable is dependent *)
80
81   For[i = 1, i <= ilen, i++,
82     depPos = Min[Position[CoeffMatrix[[i]], 1, 2]];
83     If[depPos != Infinity,
84       depList[[depPos]] = 1;
85       AppendTo[depDualList, depPos];
86     ];
87   ];
88   indepList = Flatten[Position[depList, 0, 2], 1];
89   jlen1 = Length[indepList];
90   For[i = 1, i <= ilen, i++,
91     For[j = 1, j <= jlen1, j++,
92       retPoly =
93         retPoly - (CoeffMatrix[[i]][[indepList[[j]]]]*
94           Subscript[a, VeroneseCoordinates[[ indepList[[j]] ]]])*
95         VeroneseCoordinates[[ depDualList[[i]] ]];
96     ];
97   ];
98   For[j = 1, j <= jlen1, j++,
99     retPoly =
100     retPoly +
101     VeroneseCoordinates[[ indepList[[j]] ]]*
102     Subscript[a, VeroneseCoordinates[[ indepList[[j]] ]]];
103   indepListStr =
104     indepListStr <>
105     ToString[

```

```

106      Subscript[a, VeroneseCoordinates[[ indepList[[j]] ]]],
107      StandardForm ] <> " ";
108  ];
109  Print[indepListStr];
110  retPoly
111  ];
112
113  (* Given a set of nodes, find equations of degree deg_ passing through it *)
114  FindEquation[decCodeword_, variables_, deg_] := Module[{A},
115    A = Block[{Print},
116      ExtractEquations[{ IntegerDigits[decCodeword, 2, 66]}, deg]];
117    MatrixToEquations[A, variables, deg]
118  ];
119
120
121  (* EqList stores the planes that define 26 half even set of cardinality 15 *)
122  EqList = ConstantArray[0, 20];
123  For[i = 1, i <= 20, i++,
124    tmpEq = Block[{Print}, FindEquation[ GSet[[i ]], {w, x, y, z}, 1] ];
125    EqList[[ i]] = tmpEq;
126  ];
127
128  EqList = EqList /. {Subscript[a, w] -> 1, Subscript[a, x] -> 1, Subscript[a, z] -> 1, Subscript[a,
129    y] -> 1};
130
131  AppendTo[EqList,  $\tau x - y$ ];
132  AppendTo[EqList,  $\tau x + y$ ];
133  AppendTo[EqList,  $\tau y - z$ ];
134  AppendTo[EqList,  $\tau y + z$ ];
135  AppendTo[EqList,  $\tau z - x$ ];
136  AppendTo[EqList,  $\tau z + x$ ];

```

---

## MATHEMATICA 12. $\mathfrak{A}_5$ -action as projective linear transforms

---

```

1  (* Find Projective linear transform associated to a given member of G *)
2
3  ProjLinearTransform[Group_, GenRep_, groupElement_] :=
4  Module[{word = GroupElementToWord[Group, groupElement], ilen, i, ret},
5    ilen = Length[word];
6    ret = IdentityMatrix[4];
7    For[i = 1, i <= ilen, i++,
8      If[word[[i]] > 0,
9        ret = Simplify[GenRep[[ word[[i]] ]].ret],
10       ret = Simplify[Inverse[GenRep[[ -word[[i]] ]].ret];
11     ];
12  ];
13  ret
14  ];
15
16  (* Projective Linear Transform corresponding to  $\sigma$  and  $\tau$  *)
17   $\sigma$ Matrix = 1/2*{{2, 0, 0, 0}, {0,  $\tau$ ,  $-\tau'$ , 1}, {0,  $\tau'$ , -1,  $\tau$ }, {0, 1,  $-\tau$ ,  $\tau'$ }};
18   $\tau$ Matrix = 1/2*{{2, 0, 0, 0}, {0,  $-\tau'$ , 1,  $\tau$ }, {0, 1,  $-\tau$ ,  $-\tau'$ }, {0,  $\tau$ ,  $-\tau'$ , -1}};
19
20  GProjGen = { $\sigma$ Matrix,  $\tau$ Matrix};

```

```

21 GProjMatrix = {};
22
23 (* Construct the representation A_5 -> PGL(4,CC) *)
24 For[i = 1, i <= 60, i++,
25   AppendTo[GProjMatrix,
26     ProjLinearTransform[G, GProjGen, GList[[i]] ]];
27 ];

```

---

### MATHEMATICA 13. Analyze half plane sections

---

```

1 (* Find h_i by applying A_5-action to : ( w-x-y-z, F ) = (w-x-y-z, h_1^2 ) *)
2 (* Find the PGL-action sending Pi_1=(w-x-y-z) to the plane Pi_i *)
3 i = 16; (* Run this script for all i=1, ... 20 *)
4 gi = W16SpanElements[[i]][[2]];
5 pos = GroupElementPosition[G, gi];
6 Ki = GProjMatrix[[pos]];
7 hi = Simplify[h1[Inverse[Ki].{w, x, y, z}]];

```

---

### MACAULAY2 14. Setup: half plane sections

---

```

1 R = frac (QQ[t]/(t^2-t-1)); -- t = 1/2(1+sqrt(5))
2 S = R[w,x,y,z];
3
4 F = (t^2*x^2 - y^2)*(t^2*y^2-z^2)*(t^2*z^2-x^2) - 1/4*(2*t+1)* w^2 *(x^2+y^2+z^2-w^2)^2;
5
6 -- the following equations, together with the plane sections (Pi_i=0), define C_i. Namely, C_i
   = (Pi_i=h_i=0)
7
8 h1 = t^2*(x^2*y + y^2*z + z^2*x) + (x*y^2 + y*z^2 + z*x^2) + (t^2+1)*x*y*z;
9 J1 = ideal( w-x-y-z, h1);
10
11 h2 = t^2*( x^2*y - y^2*z - z^2*x) + (-x*y^2 + y*z^2 - z*x^2) + (t^2+1)*x*y*z;
12 J2 = ideal ( w+x-y+z, h2);
13
14 h4 = t^2*(-x^2*y + y^2*z - z^2*x) + (-x*y^2 - y*z^2 + z*x^2) + (t^2+1)*x*y*z;
15 J4 = ideal( w+x+y-z, h4);
16
17 h5 = t^2*(-x^2*y - y^2*z - z^2*x) + (-x*y^2 - y*z^2 - z*x^2) - (t^2+1)*x*y*z;
18 J5 = ideal( w+x+y+z, h5);
19
20 h6 = (2*t+1)*x^3 - 1/t*x*y^2 - (3*t+2)*x^2*z + (2*t+1)*y^2*z - 1/t^2*x*z^2 - 1/t*z^3;
21 J6 = ideal( w - t*x + (1/t)*z, h6);
22
23 h8 = -1/t*x^3 - 1/t^2*x^2*y - (3*t+2)*x*y^2 + (2*t+1)*y^3 + (2*t+1)*x*z^2 - 1/t*y*z^2;
24 J8 = ideal( w + 1/t*x - t*y, h8);
25
26 h9 = t^2*(-x^2*y + y^2*z + z^2*x) + (x*y^2 - y*z^2 + z*x^2) - (t^2+1)*x*y*z;

```

```

27 J9 = ideal( w-x+y-z, h9);
28
29 h10 = -(2*t+1)*x^3 + 1/t*x*y^2 + (3*t+2)*x^2*z - (2*t+1)*y^2*z + 1/t^2*x*z^2 + 1/t*z^3;
30 J10 = ideal( w + t*x - (1/t)*z, h10);
31
32 h12 = -1/t*y^3 + (1/t^2)*y^2*z - (3*t+2)*y*z^2 - (2*t+1)*z^3 + (2*t+1)*x^2*y + 1/t*x^2*z;
33 J12 = ideal( w + 1/t*y + t*z , h12);
34
35 h17 = t^2*(x^2*y - y^2*z + z^2*x) + (x*y^2 + y*z^2 - z*x^2) - (t^2+1)*x*y*z;
36 J17 = ideal( w-x-y+z, h17);
37
38 h18 = 1/t*x^3 + 1/t^2*x^2*y + (3*t+2)*x*y^2 - (2*t+1)*y^3 - (2*t+1)*x*z^2 + 1/t*y*z^2;
39 J18 = ideal( w - 1/t*x + t*y, h18);
40
41 h19 = 1/t*y^3 - (1/t^2)*y^2*z + (3*t+2)*y*z^2 + (2*t+1)*z^3 - (2*t+1)*x^2*y - 1/t*x^2*z;
42 J19 = ideal( w - 1/t*y - t*z , h19);
43
44
45 -- the remaining guys
46 h3 = -(t+1)*x^2*y + x*y^2 - x^2*z + (t+2)*x*y*z - (t+1)*y^2*z + (t+1)*x*z^2 - y*z^2;
47 J3 = ideal( w - x + y + z, h3 );
48
49 h7 = (2*t+1)*x^2*y - (1/t)*y^3 - (1/t)*x^2*z - (1/t^2)*y^2*z - t^4*y*z^2 + (2*t+1)*z^3;
50 J7 = ideal( w + (1/t)*y - t*z, h7);
51
52 h11 = 1/t*x^3 - 1/t^2*x^2*y + (2*t+1)*y^3 - 1/t*y*z^2 + t^4*x*y^2 - (2*t+1)*x*z^2
53 J11 = ideal( w - 1/t*x - t*y, h11);
54
55 h13 = t^2*(x^2*y + y^2*z - z^2*x) + (-x*y^2 + y*z^2 + z*x^2) - (t^2+1)*x*y*z;
56 J13 = ideal( w + x - y - z, h13);
57
58 h14 = 1/t*y^3 + 1/t^2*y^2*z + t^4*y*z^2 + (-2*t-1)*z^3 + (-2*t-1)*x^2*y + 1/t*x^2*z;
59 J14 = ideal( w - 1/t*y + t*z, h14);
60
61 h15 = -1/t*x^3 + 1/t^2*x^2*y + (-2*t-1)*y^3 + 1/t*y*z^2 - t^4*x*y^2 + (2*t+1)*x*z^2
62 J15 = ideal( w + 1/t*x + t*y, h15);
63
64 h16 = (2*t+1)*x^3 - (1/t)*x*y^2 + t^4*x^2*z - (2*t+1)*y^2*z - (1/t^2)*x*z^2 + 1/t *z^3;
65 J16 = ideal( w - t*x - 1/t*z, h16);
66
67 h20 = (-2*t-1)*x^3 - t^4*x^2*z + (2*t+1)*y^2*z - 1/t*z^3 + 1/t*x*y^2 + 1/t^2*x*z^2
68 J20 = ideal( w + t*x + 1/t*z, h20);
69
70 h21 = w*(x^2 + (t*x)^2 + z^2 - w^2);
71 J21 = ideal( t*x - y , h21);
72
73 h22 = w*(x^2 + (-t*x)^2 + z^2 - w^2);
74 J22 = ideal( t*x + y , h22);
75
76 h23 = w*(x^2 + y^2 + (t*y)^2 - w^2);
77 J23 = ideal( t*y - z , h23);
78
79 h24 = w*(x^2 + y^2 + (-t*y)^2 - w^2);
80 J24 = ideal( t*y + z , h24);
81
82 h25 = w*( (t*z)^2 + y^2 + z^2 - w^2);
83 J25 = ideal( t*z - x , h25);
84
85 h26 = w*( (-t*z)^2 + y^2 + z^2 - w^2);
86 J26 = ideal( t*z + x , h26);
87

```

```

88
89 -- To Check Errata : Is  $h_i^2$  belongs to the ideal of hyperplane section ?
90 -- e.g.  $h_{21}^2 \in \text{ideal}(F, t \cdot x - y)$ 

```

---



---

MACAULAY2 15. Computing  $(B_{ij})$ : the cofactor matrix

---

```

1  load "ExtendedCode_Setup.m2"
2
3  -- Case1: Cofactor Matrix associated to  $C_1+C_9+C_{17}$ 
4
5  -- Finding equation corresponding to  $B_{14}$ 
6  time J24917 = intersect(J2,J4,J9,J17) -- has two generators, one degree 3, and the other degree
7  4
8  IB14 = ideal(J24917_0) -- take degree 3 generator
9
10 IB14_0 % J19 == 0
11 IB14_0 % J12 == 0
12 -- test whether this contains  $C_{12}$  and  $C_{19}$ 
13
14 -- equation corresponding to  $B_{24}$ 
15 J11745 = intersect( J1, J17, J4, J5 );
16 gens J11745 -- two generators, with degrees 3 and 4 respectively
17 IB24 = ideal(J11745_0);
18
19 IB24_0 % J8 == 0
20 IB24_0 % J18 == 0
21 -- the cubic contains not only  $C_1, C_{17}, C_4, C_5$ , but also  $C_8$  and  $C_{18}$ 
22
23 -- equation corresponding to  $B_{34}$ 
24 J1925 = intersect( J1, J9, J2, J5 )
25 gens J1925 -- has 2 generators, only one is of degree 3
26
27 IB34 = ideal(J1925_0)
28
29 IB34_0 % J6 == 0
30 IB34_0 % J10 == 0
31
32
33 -- equation corresponding to  $B_{12}$ 
34 J1925 = intersect( J1, J9, J2, J5 )
35
36 JTmp = intersect( J1925, J12 ); -- has 3 generators of degrees 4, 4, and higher
37 JTmp2 = intersect( ideal(JTmp_0, JTmp_1), J19 ); -- has 3 generators of degree 4 and higher
38
39 IB12 = ideal(JTmp2_0) -- Take the quartic generator
40
41 IB12_0 % J1 == 0
42 IB12_0 % J9 == 0
43 IB12_0 % J2 == 0
44 IB12_0 % J5 == 0
45 IB12_0 % J12 == 0
46 IB12_0 % J19 == 0

```

```

47 IB12_0 % J8 == 0
48 IB12_0 % J18 == 0
49
50
51 -- equation corresponding to B23
52 J91724 = intersect(J9, J17, J2, J4)
53
54 JTmp = intersect(J91724, J6); -- has 3 generators of degrees 4, 4, and higher
55 JTmp2 = intersect(ideal(JTmp_0, JTmp_1), J10);
56
57 IB23 = ideal(JTmp2_0)
58
59 IB23_0 % J9 == 0
60 IB23_0 % J17 == 0
61 IB23_0 % J2 == 0
62 IB23_0 % J4 == 0
63 IB23_0 % J8 == 0
64 IB23_0 % J18 == 0
65 IB23_0 % J6 == 0
66 IB23_0 % J10 == 0
67
68
69 -- equation corresponding to B13
70 J11745 = intersect(J1, J17, J4, J5)
71
72 JTmp = intersect(J11745, J12); -- has 3 generators of degrees 4, 4, and higher
73 JTmp2 = intersect(ideal(JTmp_0, JTmp_1), J19); -- has 3 generators of degree 4 and higher
74
75 IB13 = ideal(JTmp2_0) -- Take the quartic generator
76
77
78 IB13_0 % J1 == 0
79 IB13_0 % J17 == 0
80 IB13_0 % J4 == 0
81 IB13_0 % J5 == 0
82 IB13_0 % J12 == 0
83 IB13_0 % J19 == 0
84 IB13_0 % J6 == 0
85 IB13_0 % J10 == 0

```

---

## MATHEMATICA 16. Explicit determinantal presentation

---

```

1 CofactorMatrix = ConstantArray[0, {4, 4}];
2
3 (* Diagonals are product of linear forms *)
4 CofactorMatrix[[4]][[4]] = (w - x - y - z)*(w - x + y - z)*(w - x - y + z);
5 CofactorMatrix[[1]][[1]] = (w - x - y - z)*(w + x - y + z)*(w + x + y - z)*(τ'*w - τ'^2*y - z)
6   *(τ'*w + τ'^2*y + z);
7 CofactorMatrix[[2]][[2]] = (w - x + y - z)*(w + x + y - z)*(w + x + y + z)*(τ'*w - τ'^2*x + y)
8   *(τ'*w + τ'^2*x - y);
9 CofactorMatrix[[3]][[3]] = (w - x - y + z)*(w + x - y + z)*(w + x + y + z)*(τ*w - τ^2*x + z)*(
10   τ*w + τ^2*x - z);
11
12

```



```

9  (* B_14 is the product of h1=(w-x-y-z) with cubic passing through the planar sections
10     9,17,2,4,12,19
11     Note: cubic parts are computed by Macaulay2 *)
12 CofactorMatrix[[1]][[4]] = (w - x - y - z)*(w^2*y + (2 τ+ 1) x^2*y - y^3 + (-τ - 1) w^2*z + (τ
    - 1) x^2*z + (-τ + 1) y^2*z + (-2 τ- 1) y*z^2 + (τ + 1) z^3);
13 CofactorMatrix[[2]][[4]] = (w - x + y - z)*(w^2*x - x^3 + (τ + 1) w^2*y + (τ - 1) x^2*y + (-2
    τ- 1) x*y^2 + (-τ - 1)*y^3 + (2 τ+ 1) x*z^2 + (-τ + 1)*y*z^2);
14 CofactorMatrix[[3]][[4]] = (w - x - y + z)*( w^2*x - x^3 + (2 τ' + 1) x*y^2 + τ'^2*w^2*z + (τ'
    - 1)*x^2*z + (1 - τ')*y^2*z + (-2 τ' - 1)*x*z^2 - τ'^2*z^3);
15
16 (* B_ij with j != 4 decomposes into the product of linear term and quartic *)
17 CofactorMatrix[[1]][[2]] = (w + x + y - z)*(w^4 - w^2*x^2 + τ*w^2*x*y - τ*x^3*y - 2*w^2*y^2 +
    (-2 τ+ 1)*x^2*y^2 - τ'^2*x*y^3 + y^4 - w^2*x*z + (2 τ' + 1)*x^3*z - τ'*w^2*y*z - τ^2*x^2*
    y*z - 3*x*y^2*z + (τ + 1)*y^3*z - w^2*z^2 + 2*x^2*z^2 + τ'^2*x*y*z^2 + (τ - τ')*y^2*z^2 +
    (2 τ+ 1)*x*z^3 + (-τ + 1)*y*z^3);
18 CofactorMatrix[[1]][[3]] = (w + x - y + z)*(w^4 - w^2*x^2 - w^2*x*y + (2 τ+ 1)*x^3*y - w^2*y^2
    + 2 x^2*y^2 + (2 τ' + 1)*x*y^3 + τ'*w^2*x*z - τ'*x^3*z - τ*w^2*y*z + (τ - 2)*x^2*y*z +
    τ^2*x*y^2*z + τ*y^3*z - 2*w^2*z^2 + (1 - 2 τ')*x^2*z^2 - 3*x*y*z^2 + (τ' - τ)*y^2*z^2 +
    (-τ - 1)*x*z^3 + (-τ + 2)*y*z^3 + z^4);
19 CofactorMatrix[[2]][[3]] = (w + x + y + z)*(w^4 - 2*w^2*x^2 + x^4 + τ'*w^2*x*y + (-τ - 1)*x^3*
    y - w^2*y^2 + (1 - 2 τ')*x^2*y^2 - τ'*x*y^3 + τ*w^2*x*z + (τ - 2)*x^3*z + w^2*y*z + 3 x
    ^2*y*z + τ'^2*x*y^2*z + (-2 τ- 1)*y^3*z - w^2*z^2 + (τ' - τ)*x^2*z^2 + τ^2*x*y*z^2 + 2*y
    ^2*z^2 - τ*x*z^3 + (-2 τ' - 1)*y*z^3);
20
21 (* Fix a distinguished point P=[2:1:1:1] of sextic; we use this to normalize B_ij via B_ij(P)
    =1 *)
22 Simplify[F[2, 1, 1, 1] == 0;
23 SubstituteP := {w -> 2, x -> 1, y -> 1, z -> 1};
24
25 (* Normalize & Symmetrize the matrix *)
26 normalFactor = ConstantArray[0, {4, 4}];
27 For[i = 1, i <= 4, i++,
28   For[j = 1, j <= 4, j++,
29     normalFactor[[i]][[j]] = Simplify[CofactorMatrix[[i]][[j]] /. SubstituteP];
30     Print["Normal Factor at (", i, ",", j, ") = ", normalFactor[[i]][[j]]];
31     normalFactor[[j]][[i]] = normalFactor[[i]][[j]];
32     CofactorMatrix[[i]][[j]] = Expand[CofactorMatrix[[i]][[j]]/normalFactor[[i]][[j]]];
33     CofactorMatrix[[j]][[i]] = CofactorMatrix[[i]][[j]];
34   ];
35 ];
36
37 (* Construct the matrix (a_ij) from (B_ij) *)
38
39 (* Take the minors *)
40 Aij = Simplify[Map[Reverse, Minors[CofactorMatrix, 3], {0, 1}]];
41
42 (* Get rid of the redundant factor (F^2) *)
43 A = ConstantArray[0, {4, 4}];
44 For[i = 1, i <= 4, i++,
45   For[j = 1, j <= 4, j++,
46     tmpList =
47       Simplify[(-1)^(i+j) * PolynomialReduce[Aij[[i]][[j]], {F[w, x, y, z]^2}, {w, x, y, z}]];
48     A[[i]][[j]] = FullSimplify[tmpList[[1]][[1]]];
49   ];
50 ];
51
52 (* Then, symmetrize *)
53 For[i = 1, i <= 4, i++,
54   For[j = 1, j < i, j++,
55     A[[i]][[j]] = A[[j]][[i]];

```

```

56     ];
57     ];
58
59     (* the determinant is F (up to constant multiple) *)
60     FullSimplify [PolynomialReduce[Det[A], {F[w, x, y, z]}, {w, x, y, z}]]

```

---

### 2.3. General sextic with 65 nodes.

The scripts in this part support *Part 4*, §2 in [2]. Scripts 17–19 correspond to computer-assisted proofs in §2.2, and Scripts 20–21 are about Segre subcodes, which belong to §2.4.

---

#### MATHEMATICA 17. Finding $\{v_i\}$ for $31 = 15 + 15 + 15$

---

```

1
2  (* Finding generating set for the algebra R by base point analysis: the case 31 = 15+15+15 *)
3  Block[{Print}, W31Set = kSpan[W16Set, 3, 32]];
4  (* Half even sets of cardinality 31 that admit 15+15+15 decomposition *)
5  Orbits = OrbitDecompose[W31Set, GMatrix];
6  (* Decompose it into A_5-orbits *)
7  Length[Orbits] == 26
8
9  (* Every 31=15+15+15 contains desired basis for arbitrary 65-nodal surfaces
10  Recall the claim) if N = N_a + N_b + N_c is a 15+15+15 decomposition, then N admits
11  15+15+15+15+15 decomposition which contains N_a (resp. N_b, N_c) *)
12  flg = True;
13  For[i = 1, i <= 26, i++,
14  (* Pick one representative in each orbit, and decompose into 15+15+15 *)
15  PivotList = Flatten[FindDecompositions[Orbits[[i]][[1]], W16Set, 3]];
16  (* collect all 15+15+15+15+15 decomposition *)
17  decomp5 = FindDecompositions[Orbits[[i]][[1]], W16Set, 5];
18  For[j = 1, j <= 3, j++,
19  (* Check whether each 15+15+15+15+15 decomposition contains N_a (resp. N_b, N_c) *)
20  tmpList = Select[decomp5, MemberQ[PivotList[[j]]]];
21  If[Length[tmpList] == 0, flg = False];
22  ];
23  flg==True (* returns True, verifying the claim *)

```

---



---

#### MATHEMATICA 18. $31 = 15 + 24$ . Decomposition into orbits

---

```

1  (* Recall: ProperEven24 is the list of even sets of cardinality 24 which do not admit 15+15
2  decomposition *)
3  tmpSpanlist = {};
4
5  (* Pick an element and take its orbit *)
6  tmpwordB = IntegerDigits[ProperEven24[[1]], 2, 66];
7  Proper24B = GOrbit[{tmpwordB}, GMatrix, tmpSpanlist];

```

```

7
8  (* Remove the orbit from ProperEven24 *)
9  Proper24AC = Complement[ProperEven24, Proper24B];
10
11  (* Again, pick an element and take its orbit *)
12  tmpwordA = IntegerDigits[Proper24AC[[1]], 2, 66];
13  Proper24A = GOrbit[{tmpwordA}, GMatrix, tmpSpanlist];
14
15  (* Take the complement: The last one is also an orbit of a single element *)
16  Proper24C = Complement[Proper24AC, Proper24A];
17
18  (* Now, ProperEven24 decomposed into three orbits : Proper24A/B/C *)
19
20  (* Collect the half even sets of cardinality 31 that admit 15+24 decomposition, with 24 even
    set belonging to Proper24A *)
21  ProperJoinA = Join[Proper24A, W16Set];
22  tmp1list = Block[{Print}, kSpan[ProperJoinA, 2, 32]];
23  Proper31A = {};
24  For[i = 1, i <= Length[tmp1list], i++,
25    If[tmp1list[[i]] >= 2^65, (* Count only the half even sets *)
26      AppendTo[Proper31A, tmp1list[[i]]];
27    ];
28  ];
29
30  (* Do the same thing for the other orbits*)
31  ProperJoinB = Join[Proper24B, W16Set];
32  tmp1list = Block[{Print}, kSpan[ProperJoinB, 2, 32]];
33  Proper31B = {};
34  For[i = 1, i <= Length[tmp1list], i++,
35    If[tmp1list[[i]] >= 2^65, (* Count only the half even sets *)
36
37      AppendTo[Proper31B, tmp1list[[i]]];
38    ];
39  ];
40  ProperJoinC = Join[Proper24C, W16Set];
41  tmp1list = Block[{Print}, kSpan[ProperJoinC, 2, 32]];
42  Proper31C = {};
43  For[i = 1, i <= Length[tmp1list], i++,
44    If[tmp1list[[i]] >= 2^65, (* Count only the half even sets *)
45
46      AppendTo[Proper31C, tmp1list[[i]]];
47    ];
48  ];
49
50  (* Given set of codewords, decompose them into G-orbits *)
51  OrbitDecompose[decWords_, GMatrix_] :=
52  Module[{ret = {}, Orbit = {}, tmpWords = decWords, tmpSpanlist = {}},
53    While[tmpWords != {},
54      tmpword = IntegerDigits[tmpWords[[1]], 2, 66];
55      Orbit = GOrbit[{tmpword}, GMatrix, tmpSpanlist];
56      AppendTo[ret, Orbit];
57      tmpWords = Complement[tmpWords, Orbit];
58    ];
59    ret
60  ];
61
62  (* These are the A_5 orbits of half even sets of cardinality 31=15+24 *)
63  OrbitsA = OrbitDecompose[Proper31A, GMatrix];
64  OrbitsB = OrbitDecompose[Proper31B, GMatrix];
65  OrbitsC = OrbitDecompose[Proper31C, GMatrix];

```

---

MATHEMATICA 19. Finding  $\{v_i\}$  for  $31 = 15 + 24$ 


---

```

1  (* testword = OrbitsA[[1]][[1]] *)
2  FindDecompositions[OrbitsA[[1]][[1]], ProperJoin, 2];
3  {quadindex, linindex} = Flatten[%];
4  linindex = linindex - 65;
5  (* The testword is the sum of ProperEven24[[quadindex]] and W16Set[[linindex]] *)
6
7  decompSet = FindDecompositions[OrbitsA[[1]][[1]], W16Set, 5];
8  (* produces the list of all possible 15+15+15+15+15 decomposition
9     In this example,
10 { {1, 2, 12, 13, 17}, {1, 4, 9, 13, 19}, {1, 7, 9, 10, 25}, {1, 7, 17, 18, 22},
11   {2, 5, 6, 7, 25}, {2, 6, 17, 20, 23}, {2, 7, 13, 15, 21}, {3, 5, 21, 22, 24},
12   {3, 5, 23, 25, 26}, {3, 7, 9, 11, 21}, {3, 7, 17, 20, 26}, {4, 5, 7, 8, 22},
13   {4, 7, 13, 16, 26}, {4, 8, 9, 11, 24}, {6, 7, 11, 16, 18}, {6, 8, 11, 14, 20},
14   {7, 8, 10, 15, 20}, {10, 14, 15, 16, 18}, {10, 16, 19, 25, 26}, {12, 14, 19, 23, 24},
15   {12, 15, 18, 21, 22} }
16  *)
17
18  (* Sum of codewords, without mod out by 2 : too detect intersections of two (or more)
19     codewords *)
20  char0Sum[codewords_, sublist_] :=
21  Module[{subcode = IntegerDigits[codewords[[sublist]], 2, 66], ret,
22         i, ilen},
23    ret = subcode[[1]];
24    ilen = Length[subcode];
25    For[i = 2, i <= ilen, i++,
26      ret = ret + subcode[[i]];
27    ];
28    ret
29  ];
30  (* Find the intersection of two half even sets *)
31  char0Sum[ProperJoin, {quadindex, 65 + linindex}];
32  basenodes = Flatten[Position[%, 2]]
33  (* The decomposition 15+24 intersect at 4 nodes (so that  $31 = 15 + 24 - 2*4$ ) *)
34
35  vBasis = decompSet[{{3, 1, 20}}]; (* Take three suitable 15+15+15+15+15 decomposition *)
36  For[i = 1, i <= Length[vBasis], i++,
37    char0sum = char0Sum[W16Set, vBasis[[i]]];
38    Print[char0sum[[basenodes]]]; (* And check their vanishing orders at 4 points *)
39  ];
40  (* In this example, three decompositions give vanishing orders (2,2,2,2), (0,0,2,2), (0,0,0,0)
    respectively, showing that these are desired choices *)

```

---

## MATHEMATICA 20. Segre subcodes of Barth's code

---

```

1  (* Segre subcodes and presentations *)
2
3  (* Find all Segre subcode candidates *)
4  countList = {1, 2, 3, 4, 5, 6};
5  SegreSubcodeCandidate = {};
6  While[countList[[1]] <= 26,
7    If[Total[Mod[Total[W16BinSet[[countList]], 2]] == 0,

```

```

8     AppendTo[SegreSubcodeCandidate, countList];
9 ];
10    countList = CountNext[countList, 26];
11 ];
12
13 (* All these candidates are indeed Segre subcodes *)
14 subcode = W16BinSet[[SegreSubcodeCandidate[[-1]]]]; (* Take the "standard" Segre subcode *)
15 SortedSegreSubcode = Transpose[Sort[Transpose[subcode]]];
16 (* rearrange nodes to get a "standard model" of Segre subcodes *)
17 IsAllSegre = True;
18 For[i = 1, i <= Length[SegreSubcodeCandidate] - 1, i++,
19     subcode = W16BinSet[[ SegreSubcodeCandidate[[i]] ]];
20     SortedSegreCandidate = Transpose[Sort[Transpose[subcode]]];
21     IsAllSegre = IsAllSegre && ( SortedSegreSubcode == SortedSegreCandidate);
22     (* compare with "standard model" *)
23 ];
24 IsAllSegre (* returns True if each candidate is a Segre subcode *)
25
26 (* On Segre Configurations *)
27 DegenerateConfigs = {};
28 For[i = 1, i <= Length[SegreSubcodeCandidate], i++,
29     SegrePlanes = EqList[[ SegreSubcodeCandidate[[i]] ]];
30     Coeffs = D[SegrePlanes, {{w, x, y, z}, 1}];
31     If[MatrixRank[Coeffs] < 4, AppendTo[DegenerateConfigs, i]];
32 ];
33 DegenerateConfigs (* returns {65}, which is the standard one *)

```

---

## MATHEMATICA 21. Explicit Barth's equation from Segre subcodes

---

```

1 (* Take the product of six planes *)
2 i = 1;
3 planeprod =
4     Product[EqList[[SegreSubcodeCandidate[[i, j]]]], {j, 1, 6}];
5
6 F[w_, x_, y_, z_] := (τ^2 x^2 - y^2) ( τ^2 y^2 - z^2 ) ( τ^2 z^2 - x^2 ) - (2 τ+ 1)/4 * w^2 (
7     x^2 + y^2 + z^2 - w^2 )^2;
8 (* Introduce a parameter "a": F equals planeprod + (cubic)^2, but there is an ambiguity by
9     constant multiple *)
10 Clear[a];
11
12 (* Take heuristic substitution to make computation simpler *)
13 subs = {x -> 1, y -> τ, z -> 1};
14 g = ExpandAll[F[w, x, y, z] - a*planeprod] /. subs;
15 dg = D[g, {w, 1}];
16
17 (* If "g" is perfect square, then the resultant Res_w(g,dg) must be zero *)
18 res = Resultant[g, dg, w]
19 Solve[res == 0, a]
20
21 (* Choose reasonable candidate of "a" from the above solution *)
22 a = 1/4*τ;
23 g = ExpandAll[F[w, x, y, z] - a*planeprod]; (* redefine g (neutralize substitution) *)
24
25 Factor[g, Extension -> {τ, τ'}] (* The resulting polynomial is a perfect square *)

```



## 3. MAGMA SCRIPTS BY MICHAEL KIERMAIER

The following program classifies the node-secants of the Barth sextic. It verifies the group of linear automorphisms of the Barth sextic and the connection to the Doro-Hall graph. Moreover, several coding theoretic properties of the Barth code are computed. The related computations were carried out in *Part 4, §3* in [2].

## MAGMA 22. Coding-theoretic properties of Barth codes

---

```

1  QX := PolynomialRing(Rationals());
2  fgolden := QX.1^2 - QX.1 - 1; // defining polynomial of the golden ratio
3  // roots of fgolden: golden ratio tau = (1 + sqrt(5))/2, ta2 = 1 - tau = (1 - sqrt(5))/2
4  // we have tau + ta2 = 1, tau * ta2 = -1 and +- sqrt(5) = 2*tau - 1
5  Qgolden<tau> := ext<Rationals() | fgolden >; // roots: tau, ta2 := 1 - tau;
6  ta2 := 1 - tau;
7  QgoldenP3<w0,w1,w2,w3> := ProjectiveSpace(Qgolden,3); // ambient space for the Barth sextic
8  fBarth := (tau^2*w1^2 - w2^2)*(tau^2*w2^2 - w3^2)*(tau^2*w3^2 - w1^2) - 1/4*(2*tau+1)*w0^2*(w1
    ^2+w2^2+w3^2-w0^2)^2; // defining polynomial of the Barth sextic
9  F := Surface(QgoldenP3, fBarth); // Barth sextic
10
11  Vnodes := VectorSpace(Qgolden,4); // ambient space for the nodes
12
13  // enter the nodes manually to force the same order as in the article.
14  A_12_34 := sub<Vnodes | [0, 1, tau, -ta2]>;
15  A_41_25 := sub<Vnodes | [0, 1, -tau, ta2]>;
16  A_31_52 := sub<Vnodes | [0, 1, -tau, -ta2]>;
17  A_51_34 := sub<Vnodes | [0, 1, tau, ta2]>;
18
19  A_12_53 := sub<Vnodes | [0, -ta2, 1, tau]>;
20  A_41_53 := sub<Vnodes | [0, ta2, 1, tau]>;
21  A_31_24 := sub<Vnodes | [0, ta2, 1, -tau]>;
22  A_51_42 := sub<Vnodes | [0, -ta2, 1, -tau]>;
23
24  A_12_45 := sub<Vnodes | [0, tau, -ta2, 1]>;
25  A_41_32 := sub<Vnodes | [0, -tau, -ta2, 1]>;
26  A_31_45 := sub<Vnodes | [0, tau, ta2, 1]>;
27  A_51_23 := sub<Vnodes | [0, -tau, ta2, 1]>;
28
29  A_23_45 := sub<Vnodes | [0, 1, 0, 0]>;
30  A_25_34 := sub<Vnodes | [0, 0, 1, 0]>;
31  A_24_35 := sub<Vnodes | [0, 0, 0, 1]>;
32
33  nodes_A := [
34      A_12_34,
35      A_41_25,
36      A_31_52,
37      A_51_34,
38      A_12_53,
39      A_41_53,
40      A_31_24,
41      A_51_42,
42      A_12_45,
43      A_41_32,
44      A_31_45,
45      A_51_23,
46      A_23_45,
47      A_25_34,
48      A_24_35
49  ];

```

```

50 // A5-orbit of length 15
51 // nodes_A are contained in the plane <e2, e3, e4>.
52
53 B_1_2_34 := sub<Vnodes | [2, 1, tau, -ta2]>;
54 B_4_1_25 := sub<Vnodes | [2, -1, tau, -ta2]>;
55 B_3_1_52 := sub<Vnodes | [2, 1, -tau, -ta2]>;
56 B_5_1_34 := sub<Vnodes | [2, 1, tau, ta2]>;
57
58 B_2_1_43 := sub<Vnodes | [2, -1, -tau, ta2]>;
59 B_1_4_52 := sub<Vnodes | [2, 1, -tau, ta2]>;
60 B_1_3_25 := sub<Vnodes | [2, -1, tau, ta2]>;
61 B_1_5_43 := sub<Vnodes | [2, -1, -tau, -ta2]>;
62
63 B_1_2_53 := sub<Vnodes | [2, -ta2, 1, tau]>;
64 B_4_1_53 := sub<Vnodes | [2, ta2, 1, tau]>;
65 B_3_1_24 := sub<Vnodes | [2, -ta2, -1, tau]>;
66 B_5_1_42 := sub<Vnodes | [2, -ta2, 1, -tau]>;
67
68 B_2_1_35 := sub<Vnodes | [2, ta2, -1, -tau]>;
69 B_1_4_35 := sub<Vnodes | [2, -ta2, -1, -tau]>;
70 B_1_3_42 := sub<Vnodes | [2, ta2, 1, -tau]>;
71 B_1_5_24 := sub<Vnodes | [2, ta2, -1, tau]>;
72
73 B_1_2_45 := sub<Vnodes | [2, tau, -ta2, 1]>;
74 B_4_1_32 := sub<Vnodes | [2, -tau, -ta2, 1]>;
75 B_3_1_45 := sub<Vnodes | [2, tau, ta2, 1]>;
76 B_5_1_23 := sub<Vnodes | [2, tau, -ta2, -1]>;
77
78 B_2_1_54 := sub<Vnodes | [2, -tau, ta2, -1]>;
79 B_1_4_23 := sub<Vnodes | [2, tau, ta2, -1]>;
80 B_1_3_54 := sub<Vnodes | [2, -tau, -ta2, -1]>;
81 B_1_5_32 := sub<Vnodes | [2, -tau, ta2, 1]>;
82
83 B_2_3_45 := sub<Vnodes | [1, 1, 0, 0]>;
84 B_3_2_54 := sub<Vnodes | [1, -1, 0, 0]>;
85 B_2_5_34 := sub<Vnodes | [1, 0, 1, 0]>;
86 B_5_2_43 := sub<Vnodes | [1, 0, -1, 0]>;
87 B_2_4_53 := sub<Vnodes | [1, 0, 0, 1]>;
88 B_4_2_35 := sub<Vnodes | [1, 0, 0, -1]>;
89
90 nodes_B := [
91   B_1_2_34,
92   B_4_1_25,
93   B_3_1_52,
94   B_5_1_34,
95   B_2_1_43,
96   B_1_4_52,
97   B_1_3_25,
98   B_1_5_43,
99   B_1_2_53,
100  B_4_1_53,
101  B_3_1_24,
102  B_5_1_42,
103  B_2_1_35,
104  B_1_4_35,
105  B_1_3_42,
106  B_1_5_24,
107  B_1_2_45,
108  B_4_1_32,
109  B_3_1_45,
110  B_5_1_23,

```



```

111     B_2_1_54,
112     B_1_4_23,
113     B_1_3_54,
114     B_1_5_32,
115     B_2_3_45,
116     B_3_2_54,
117     B_2_5_34,
118     B_5_2_43,
119     B_2_4_53,
120     B_4_2_35
121 ];
122 // A5-orbit of length 30
123
124 C_1_2 := sub<Vnodes | [1, 1, 1, 1]>;
125 C_4_1 := sub<Vnodes | [1, -1, 1, 1]>;
126 C_3_1 := sub<Vnodes | [1, 1, -1, 1]>;
127 C_5_1 := sub<Vnodes | [1, 1, 1, -1]>;
128
129 C_2_1 := sub<Vnodes | [1, -1, -1, -1]>;
130 C_1_4 := sub<Vnodes | [1, 1, -1, -1]>;
131 C_1_3 := sub<Vnodes | [1, -1, 1, -1]>;
132 C_1_5 := sub<Vnodes | [1, -1, -1, 1]>;
133
134 C_5_3 := sub<Vnodes | [1, 0, -ta2, tau]>;
135 C_2_4 := sub<Vnodes | [1, 0, ta2, tau]>;
136 C_3_5 := sub<Vnodes | [1, 0, ta2, -tau]>;
137 C_4_2 := sub<Vnodes | [1, 0, -ta2, -tau]>;
138
139 C_4_5 := sub<Vnodes | [1, tau, 0, -ta2]>;
140 C_3_2 := sub<Vnodes | [1, -tau, 0, -ta2]>;
141 C_5_4 := sub<Vnodes | [1, -tau, 0, ta2]>;
142 C_2_3 := sub<Vnodes | [1, tau, 0, ta2]>;
143
144 C_3_4 := sub<Vnodes | [1, -ta2, tau, 0]>;
145 C_2_5 := sub<Vnodes | [1, ta2, tau, 0]>;
146 C_4_3 := sub<Vnodes | [1, ta2, -tau, 0]>;
147 C_5_2 := sub<Vnodes | [1, -ta2, -tau, 0]>;
148
149 nodes_C := [
150     C_1_2,
151     C_4_1,
152     C_3_1,
153     C_5_1,
154     C_2_1,
155     C_1_4,
156     C_1_3,
157     C_1_5,
158     C_5_3,
159     C_2_4,
160     C_3_5,
161     C_4_2,
162     C_4_5,
163     C_3_2,
164     C_5_4,
165     C_2_3,
166     C_3_4,
167     C_2_5,
168     C_4_3,
169     C_5_2
170 ];
171 // A5-orbit of length 20

```

```

172
173 nodes := nodes_A cat nodes_B cat nodes_C;
174
175 // double check if we have the correct set of nodes
176 if not {x : x in nodes} eq {sub<Vnodes | [x[i] : i in [1..4]]> : x in SingularPoints(F)} then
177   printf "ERROR: The provided set of nodes is not correct.";
178 end if;
179
180 function point_to_representative(point)
181   return Representative(Basis(point));
182 end function;
183
184 function matrix_from_frame_image(frame_image)
185   // the standard frame in  $F^n$  is  $[1,0,\dots,0], [0,1,\dots,0], \dots [0,0,\dots,1], [1,1,\dots,1]$ 
186   // (i.e. a projective basis)
187   // Each ordered frame is the image of a unique element of  $\text{PGL}(F^n)$ .
188   // This function computes a matrix representative of that mapping (operating from the
189     right),
190   // which is unique up to scaling.
191   // The input 'frame_image' is expected as a sequence of  $n+1$  vectors in  $F^n$ 
192
193   // Let frame_image =  $[b_1 \dots b_{(n+1)}]$ 
194   // Let  $a_1 \dots a_n$  be the rows of the sought-after matrix A.
195   // and let B be the matrix with the rows  $b_1 \dots b_n$ 
196   // From  $\langle e_i \rangle \rightarrow \langle a_i \rangle$  we have  $a_i = \lambda_{b,i} b_i$  with  $\lambda_{b,i}$  in  $F$ .
197   // Now  $\langle [1,1,\dots,1] \rangle \rightarrow \langle A*[1,1,\dots,1] \rangle = \langle \lambda_{b,1} b_1 + \dots + \lambda_{b,n} b_n \rangle$ 
198   // which must equal  $\langle b_{(n+1)} \rangle$ 
199   // So  $(\lambda_{b,1} \dots \lambda_{b,n}) B = b_{(n+1)}$  (up to scaling)
200   //  $\Leftrightarrow (\lambda_{b,1} \dots \lambda_{b,n}) = b_{(n+1)} B^{-1}$ 
201
202   n := #frame_image-1;
203   frame_image_vec := [point_to_representative(pt) : pt in frame_image];
204   F := Parent(frame_image_vec[1][1]);
205   B := Matrix(F,n,n,[ElementToSequence(frame_image_vec[i]) : i in [1..n]]);
206   lambda := frame_image_vec[n+1] * B^(-1);
207   A := Matrix(F,n,n,[ElementToSequence(lambda[i]*frame_image_vec[i]) : i in [1..n]]);
208
209   return A;
210 end function;
211
212 function is_frame(points)
213   if Dimension(&+points) ne #points-1 then return false; end if;
214   for i := 1 to #points do
215     if Dimension(&+[points[j] : j in [1..#points] | j ne i]) ne #points-1 then return false;
216     end if;
217   end for;
218   return true;
219 end function;
220
221 function linear_automorphisms_of_set_of_nodes()
222   res_mat := {};
223   res_perm := {};
224   nodes_indexed := IndexedSet(nodes);
225   co := 0;
226   frame := [A_23_45, A_25_34, A_24_35, C_1_2, C_2_1];
227   S1 := (matrix_from_frame_image(frame))^(-1);
228   if not is_frame(frame) then print "ERROR: the chosen points do not form a projective frame"
229     ; end if;
230
231   // there are exactly 6 straight lines containing 5 nodes.
232   // they span the plane consisting of the points  $[0 * * *]$ .
233   // therefore, this plane is distinguished and must be mapped to itself.

```

```

230 // the set of nodes of type A equals the set of nodes contained in that plane.
231 // hence a node of type A must be mapped to a node of type A,
232 // and a node of type B or C must again be mapped to a node of type B or C.
233 for im1 in nodes_A do
234   for im2 in nodes_A do
235     if Dimension(im1 + im2) ne 2 then continue im2; end if;
236     for im3 in nodes_A do
237       if Dimension(im1 + im2 + im3) ne 3 then continue im3; end if;
238       for im4 in nodes_B cat nodes_C do
239         if Dimension(im1 + im2 + im3 + im4) ne 4 then continue im4; end if;
240         for im5 in nodes_B cat nodes_C do
241           frame_image := [im1, im2, im3, im4, im5];
242           if not is_frame(frame_image) then continue im5; end if;
243           co += 1;
244           S2 := matrix_from_frame_image(frame_image);
245           S := S1 * S2;
246           perm := [];
247           for v in nodes do
248             v_im_index := Index(nodes_indexed, sub<Vnodes | point_to_representative(v) *
249                                   S>);
250             if v_im_index eq 0 then
251               // image of v is not a node ==> no automorphism
252               continue im5;
253             else
254               Append(~perm, v_im_index);
255             end if;
256           end for;
257           // automorphism found
258           Include(~res_mat, S);
259           Include(~res_perm, SymmetricGroup(#nodes)!perm);
260         end for;
261       end for;
262     end for;
263   end for;
264   return sub<GL(Dimension(Vnodes), BaseRing(Vnodes)) | res_mat>, sub<SymmetricGroup(#nodes) |
265     res_perm>;
266 end function;
267
268 // enter the permutations sigma and tau as provided in the article.
269 perm_sigma := SymmetricGroup(65)!
270 // sigma_A
271 (1,10,7)(2,15,4)(3,5,12)(6,8,14)(9,13,11)
272 // sigma_B
273 (1+15,22+15,11+15)(2+15,30+15,8+15)(3+15,9+15,20+15)(4+15,6+15,29+15)(5+15,18+15,15+15)
274 (7+15,13+15,24+15)(10+15,12+15,28+15)(14+15,16+15,27+15)(17+15,25+15,19+15)
275 (21+15,26+15,23+15)
276 // sigma_C
277 (1+45,16+45,3+45)(2+45,12+45,19+45)(4+45,20+45,9+45)(5+45,14+45,7+45)(6+45,10+45,17+45)
278 (8+45,18+45,11+45);
279
280 perm_tau := SymmetricGroup(65)!
281 // tau_A
282 (1,11)(3,14)(4,7)(5,13)(6,10)(12,15)
283 // tau_B
284 (1+15,19+15)(2+15,6+15)(3+15,27+15)(4+15,11+15)(5+15,23+15)(7+15,28+15)(8+15,15+15)
285 (9+15,25+15)(10+15,22+15)(12+15,16+15)(13+15,26+15)(14+15,18+15)(20+15,29+15)
286 (24+15,30+15)
287 // tau_C
288 (1+45,13+45)(2+45,6+45)(3+45,17+45)(4+45,10+45)(5+45,15+45)(7+45,19+45)(8+45,12+45)
289 (9+45,16+45)(11+45,14+45)(18+45,20+45);

```

```

283
284 function perm_negate(pos)
285     indices := [];
286     for nd in nodes do
287         nd_neg := point_to_representative(nd);
288         nd_neg[pos] := -1;
289         nd_neg := sub<Vnodes | nd_neg>;
290         for i:=1 to #nodes do
291             if nodes[i] eq nd_neg then
292                 Append(~indices,i);
293                 continue nd;
294             end if;
295         end for;
296     end for;
297     return SymmetricGroup(#nodes)!indices;
298 end function;
299
300 group_A5 := sub<SymmetricGroup(#nodes) | perm_sigma, perm_tau>;
301 group_Z2_3 := sub<SymmetricGroup(#nodes) | perm_negate(2), perm_negate(3), perm_negate(4)>;
302 group_120 := sub<SymmetricGroup(#nodes) | group_A5, group_Z2_3>;
303
304 generator_matrix_barth_code_extended := Matrix(GF(2),13,66,[
305 // extended code assigned to the Barth sextic, as computed in the article.
306 // the additional column is the first one.
307 1,0,0,0,0,0,0,0,0,1,1,0,0,0,1,0,0,0,0,0,1,1,0,1,0,0,0,0,0,0,1,0,0,0,1,1,0,0,0,
308   1,1,1,1,1,1,1,0,0,1,1,1,1,0,0,1,1,1,1,0,0,1,0,1,0,
309 0,1,0,0,0,0,0,0,1,0,0,0,1,0,1,0,0,0,0,0,1,1,1,0,0,0,0,0,1,0,1,1,1,0,0,0,0,1,
310   1,0,0,1,1,0,1,1,0,0,0,1,0,0,1,0,1,1,0,0,0,1,0,1,0,0,
311 0,0,1,0,0,0,0,0,1,0,1,1,1,1,1,0,0,0,0,1,0,1,1,1,0,0,0,0,1,0,1,1,1,0,1,0,0,1,
312   1,0,0,1,1,0,0,0,1,0,0,0,0,0,1,1,0,1,1,0,1,1,0,1,1,1,0,1,1,0,1,0,0,1,
313 0,0,0,1,0,0,0,0,1,0,0,1,0,0,0,1,0,0,0,0,0,1,1,1,1,0,0,0,0,1,0,1,0,0,0,1,1,0,1,0,
314   1,0,1,0,1,0,1,0,0,1,1,0,0,0,0,0,1,0,1,0,0,0,1,0,1,1,0,0,0,0,1,1,0,1,0,
315 0,0,0,0,1,0,0,0,1,0,1,0,0,1,0,0,0,0,0,0,1,1,0,1,0,0,0,1,0,1,1,0,0,0,0,1,1,1,0,
316   0,1,0,1,0,1,0,0,0,1,0,1,0,0,0,0,0,1,0,1,0,0,0,1,0,1,0,0,0,1,0,1,0,1,1,
317 0,0,0,0,0,0,0,0,0,0,0,0,0,0,0,0,0,0,0,0,0,1,0,0,0,0,0,1,0,0,0,1,1,0,0,0,1,0,0,0,
318   1,1,1,1,1,1,1,0,1,1,0,1,1,0,1,1,0,1,0,0,1,0,1,1,0,0,1,0,1,0,1,0,
319 0,0,0,0,0,0,0,0,0,0,0,0,0,0,0,0,0,0,0,0,0,1,0,0,0,1,0,0,0,0,0,1,0,0,0,1,0,0,0,1,0,
320   1,1,1,1,1,1,0,1,1,1,0,1,1,1,0,1,0,1,0,1,0,1,0,1,0,1,0,1,0,1,0,1,0,1,0,1,0,1,0,1,
321 ]);
322
323 K_extended := LinearCode(generator_matrix_barth_code_extended);
324 K := ShortenCode(K_extended,1);
325
326 // subspaces spanned by the coordinates of the orbits A, B and C
327 space_ABC := [Rowspace(M) : M in <
328     HorizontalJoin(ScalarMatrix(GF(2),15,1),ZeroMatrix(GF(2),15,30+20)),
329     HorizontalJoin(<ZeroMatrix(GF(2),30,15),ScalarMatrix(GF(2),30,1),ZeroMatrix(GF(2),30,20)>),
330     HorizontalJoin(ZeroMatrix(GF(2),20,15+30),ScalarMatrix(GF(2),20,1))
331 >];

```

```

331
332 QgoldenX2<X,Y> := PolynomialRing(Qgolden,2);
333
334 function type_of_pair_of_nodes(pair)
335     // Let x,y be two different nodes of the Barth sextic.
336     // the pair (x,y) is classified into one of the following types, by looking at the straight
337     // line L through x and y:
338     // Type X (encoded by 1): L intersects the Barth sextic in two further points of
339     //     multiplicity 1
340     //     over Qgolden: factorization of type  $x^2 y^2 a^1 b^1$  or of type  $x^2 y^2 f$  where  $f$  is
341     //     irreducible of degree 2)
342     // Type Y (encoded by 3): L intersects the Barth sextic in a single further point of
343     //     multiplicity 2 ( $x^2 y^2 a^2$ )
344     // Type Z (encoded by +2 or -2): intersection multiplicities are  $x^4 y^2$  (type Z+) and  $x^2$ 
345     //      $y^4$  (type Z-)
346     // Type 0: L is contained in the Barth sextic
347     if not #pair eq 2 then
348         printf "ERROR: type_of_pair_of_nodes must be passed a pair of nodes";
349     end if;
350     x := pair[1];
351     y := pair[2];
352     for z in [x,y] do
353         if not (z in nodes) then
354             printf "ERROR: %o is not a node\n", z;
355         end if;
356     end for;
357     if x eq y then
358         printf "ERROR: type_of_pair_of_nodes has been called with twice the same node %o\n", x;
359     end if;
360     f := Evaluate(fBarth, [X*point_to_representative(p1)[i]+Y*point_to_representative(p2)[i] : i
361         in [1..4]]); // compute intersection polynomial
362     if f eq 0 then // type 0
363         return "0";
364     else
365         if not (Degree(f) eq 6) then
366             print "ERROR: degree of the intersection polynomial should be 6";
367         end if;
368         f := ExactQuotient(f,X^2 * Y^2); // remove the obvious factors (both X and Y are nodes
369             // => they are of multiplicity >= 2)
370         if IsDivisibleBy(f,X^2) then // type Z+
371             return "Z+";
372         elif IsDivisibleBy(f,Y^2) then // type Z-
373             return "Z-";
374         elif IsDivisibleBy(f,X) or IsDivisibleBy(f,Y) then
375             print "ERROR: the pair of nodes %o and %o does not yield one of the claimed types.\n",X,Y;
376         else ffact := Factorization(f);
377             if
378                 (#ffact eq 1 and Degree(ffact[1][1]) eq 2 and ffact[1][2] eq 1)
379                 // single factor of degree 2 => f is irreducible over perfect field Qgolden => f
380                 // separable => type X
381             or
382                 (#ffact eq 2 and Degree(ffact[1][1]) eq 1 and Degree(ffact[2][1]) eq 1 and
383                 ffact[1][2] eq 1 and ffact[2][2] eq 1)
384                 // two different factors of degree 1 => type Y
385             then
386                 return "X";
387             elif (#ffact eq 1) and (Degree(ffact[1][1]) eq 1) and (ffact[1][2] eq 2) then //
388                 double factor of degree 1 => type Y
389                 return "Y";
390             else

```

```

382         print "ERROR: the pair of nodes %o and %o does not yield one of the claimed types.\
           n",X,Y;
383     end if;
384 end if;
385 end if;
386 end function;
387
388 function barth_sextic_to_graph()
389     return Graph<#nodes | {e : e in Subsets({1..#nodes},2) | type_of_pair_of_nodes([nodes[a] :
           a in e]) eq "X"}>;
390 end function;
391
392 function is_local_petersen_graph(Gr)
393     // construct Petersen graph as the Kneser graph K(5,2)
394     pairs := Subsets({1..5},2);
395     edges := {e : e in Subsets(pairs,2) | IsEmpty(&meet e)};
396     petersen_graph := Graph<SetToIndexedSet(pairs) | edges>;
397
398     for v in Vertices(Gr) do
399         sphere := sub<Gr | Neighbors(v)>;
400         if not IsIsomorphic(sphere,petersen_graph) then
401             return false;
402         end if;
403     end for;
404     return true;
405 end function;
406
407 function sphere(vert,dist)
408     return {e : e in Parent(vert) | Distance(vert,e) eq dist};
409 end function;
410
411 function vertex_set_to_characteristic_vector(vertset)
412     v := #Universe(vertset);
413     return Vector(GF(2),[ i in vertset select 1 else 0 : i in [1..v] ]);
414 end function;
415
416 function code_to_orbits(C,group)
417     return Orbits(group,GSet(group,{c : c in C}));
418 end function;
419
420 function codeword_orbits_to_stats(orb)
421     stats := [];
422     for o in orb do
423         Append(~stats,<Weight(Representative(o)), #o>);
424     end for;
425     Sort(~stats,func<x,y | x[1] - y[1]>);
426     return stats;
427 end function;
428
429 function binary_code_to_permutation_module(C,group)
430     full_permutation_module := PermutationModule(group,GF(2));
431     return sub<full_permutation_module | RowSpace(GeneratorMatrix(C))>;
432 end function;
433
434 procedure print_submodules_info(C,group)
435     full_permutation_module := PermutationModule(group,GF(2));
436     CM := sub<full_permutation_module | RowSpace(GeneratorMatrix(C))>;
437     CMsub := Submodules(CM);
438     index_nontriv := [i : i in [1..#CMsub] | Dimension(CMsub[i]) ne 0];
439     for i in index_nontriv do
440         if i eq 1 then continue i; end if;

```

```

441     submodule_space := sub<VectorSpace(GF(2),65) | [ElementToSequence(
442         full_permutation_module!v) : v in Generators(CMsub[i])]>;
443     printf "submodule #%-o: dimension %o.",i,Dimension(CMsub[i]);
444     for j := 1 to 3 do
445         J := Exclude({1,2,3},j);
446         if submodule_space eq (&+[space_ABC[jj] : jj in J] meet RowSpace(GeneratorMatrix(C)))
447             then
448             printf " equals ker_%o.", "ABC"[j];
449             end if;
450         end for;
451         if IsIrreducible(CMsub[i]) then
452             printf " irreducibe";
453         else
454             printf " contains submodules #";
455             for j in index_nontriv do if
456                 CMsub[j] subset CMsub[i] then
457                     printf " %o",j;
458                 end if;
459             end for;
460             printf ". weight distribution %o\n",WeightDistribution(LinearCode(submodule_space));
461         end for;
462     end procedure;
463
464     printf "The %o nodes will be considered in the following order.\n", #nodes;
465     for i := 1 to #nodes do
466         printf "node #%-o: %o\n",i,point_to_representative(nodes[i]);
467     end for;
468
469     g_barth_mat, g_barth_perm := linear_automorphisms_of_set_of_nodes();
470
471     printf "The group of linear automorphisms of the set of nodes is of size...%o.\n",#
472         g_barth_perm;
473     printf "It is isomorphic to a direct product of A_5 x Z/2Z...%o.\n",IsIsomorphic(g_barth_perm,
474         DirectProduct(SymmetricGroup(2),AlternatingGroup(5)));
475     printf "It is spanned by the sign changes and by the permutations sigma and tau as given in
476         the article...%o.\n",g_barth_perm eq group_120;
477
478     printf "Generator matrix of the extended code K' as computed in the article (the first column
479         corresponds to the extension):\n%o\n", generator_matrix_barth_code_extended;
480
481     printf "Aut(K) is isomorphic to PSignal(2,25)...%o.\n", IsIsomorphic(AutomorphismGroup(K),
482         PSignal(2,25));
483     printf "Aut(K') is isomorphic to PSignal(2,25)...%o.\n", IsIsomorphic(AutomorphismGroup(
484         K_extended),PSignal(2,25));
485
486     printf "weight distribution of K is %o.\n", WeightDistribution(K);
487     printf "weight distribution of K' is %o.\n", WeightDistribution(K_extended);
488
489     printf "orbit structure on the codewords of K (listed as <weight, orbit length>): %o\n",
490         codeword_orbits_to_stats(code_to_orbits(K,AutomorphismGroup(K)));
491     printf "orbit structure on the codewords of K' (listed as <weight, orbit length>): %o\n",
492         codeword_orbits_to_stats(code_to_orbits(K_extended,AutomorphismGroup(K_extended)));
493
494     printf "\nstructure of the nonzero submodules of K under the A5-action:\n";
495     print_submodules_info(K,group_A5);
496
497     printf "\nstructure of the nonzero submodules of K under the full icosahedral action:\n";
498     print_submodules_info(K,group_120);
499

```

---

```

491 printf "type distribution for pairs (x,y) of nodes with fixed x in orbit A, y in A; B; C:\n%o\
      n", {[* [ {type_of_pair_of_nodes([x,y]) : y in 0 | y ne x *} : 0 in [nodes_A,nodes_B,
      nodes_C]] : x in nodes_A *};
492 printf "type distribution for pairs (x,y) of nodes with fixed x in orbit A, y in A; B; C:\n%o\
      n", {[* [ {type_of_pair_of_nodes([x,y]) : y in 0 | y ne x *} : 0 in [nodes_A,nodes_B,
      nodes_C]] : x in nodes_B *};
493 printf "type distribution for pairs (x,y) of nodes with fixed x in orbit A, y in A; B; C:\n%o\
      n", {[* [ {type_of_pair_of_nodes([x,y]) : y in 0 | y ne x *} : 0 in [nodes_A,nodes_B,
      nodes_C]] : x in nodes_C *};
494
495 barth_graph := barth_sextic_to_graph();
496 printf "The graph G given by all pairs of nodes of type X is local Petersen...%o.\n",
      is_local_petersen_graph(barth_graph);
497 printf "Hence by the classification of connected local Petersen graphs, G is isomorphic to the
      Doro-Hall graph. By its characterization as the (unique) distance regular graph with
      intersection array {10, 6, 4; 1, 2, 5}, we get that the diameter is 3, and the spheres of
      radius 1, 2, 3 are of sizes 10, 30 and 24, respectively.\n";
498 ind_nr := IndependenceNumber(barth_graph);
499 printf "The independence number of G is...%o.\n",ind_nr;
500 independent_sets := {vertex_set_to_characteristic_vector(x) : x in AllCliques(Complement(
      barth_graph),ind_nr)};
501 printf "There are %o independent sets of maximum size.\n",#independent_sets, ind_nr;
502 sums_of_independent_sets := {&+T : T in Subsets(independent_sets,2)};
503 printf "There are %o non-empty symmetric differences of two independent sets of maximum size.\
      n",#sums_of_independent_sets;
504 printf "The weight distribution of the set of their characteristic vectors is %o.\n",{* Weight
      (x) : x in sums_of_independent_sets *};
505 printf "These %o vectors span the code K...%o.\n",#sums_of_independent_sets,LinearCode(sub<
      VectorSpace(GF(2),#nodes) | sums_of_independent_sets>) eq K;
506 weight_24_words := Words(K,24);
507 spheres_3 := { vertex_set_to_characteristic_vector(sphere(v,3)) : v in Vertices(barth_graph)
      };
508 printf "The remaining %o words of weight 24 are precisely the characteristic vectors of the
      spheres of radius 3...%o.\n",#weight_24_words - #sums_of_independent_sets, weight_24_words
      diff sums_of_independent_sets eq spheres_3;
509 printf "These %o vectors span the code K...%o.\n",#spheres_3,LinearCode(sub<VectorSpace(GF(2)
      ,#nodes) | spheres_3>) eq K;

```

---

#### 4. MAGMA SCRIPTS BY STEPHEN COUGHLAN & DAVIDE FRAPPORTI

**4.1. Studying lines through nodes on the Barth sextic surface.** The following script examines the lines connecting two nodes of Barth sextic surface. This can be found in *Part 4*, §3.2.4 in [2]

---

##### MAGMA 23. Lines connecting two nodes of Barth sextic surface

---

```

1 // some code to work out intersections of lines through
2 // nodes on Barth sextic surface
3
4 Q:=Rationals();
5 RR<z>:=PolynomialRing(Q);
6 K<t>:=SplittingField(z^2-z-1);
7

```



```

8   tbar:=1-t;
9
10
11  R<x,y>:=PolynomialRing(K,2);
12
13
14
15  // computes multiplicities of points
16  // on the line joining nodes P and Q
17  // on Barth sextic
18
19
20
21  function intersect(P,Q)
22  mult:={* *};
23
24  w0:=x*P[1]+y*Q[1];
25  w1:=x*P[2]+y*Q[2];
26  w2:=x*P[3]+y*Q[3];
27  w3:=x*P[4]+y*Q[4];
28
29  F := (t^2*w1^2 - w2^2)*(t^2*w2^2 - w3^2)*(t^2*w3^2 - w1^2)
30      - 1/4*(2*t + 1)*(w1^2 + w2^2 + w3^2 - w0^2)^2*w0^2;
31
32
33  if F ne 0 then
34
35      // return multiset containing
36      // multiplicities of points on line
37
38      Fac:=Factorization(F);
39
40      for m in Fac do
41
42          Include(~mult,m[2]^Degree(m[1]));
43
44      end for;
45
46      return mult;
47
48  else
49
50      // line contained in surface
51      return {* 0 *};
52
53  end if;
54
55  end function;
56
57  /*
58  // this stuff can be used to compute points more
59  // precisely if necessary
60
61  pts:=Points(Scheme(Proj(R),m[1]));
62
63  for p in pts do
64
65      p[1]*P[1]+p[2]*Q[1],
66      p[1]*P[2]+p[2]*Q[2],
67      p[1]*P[3]+p[2]*Q[3],
68      p[1]*P[4]+p[2]*Q[4];

```

```

69
70     end for;
71
72
73
74
75 // for example, to check tangency at a point, can either
76 // compute derivatives at that point or can check whether
77 // the given point is one of the nodes (considering the
78 // coordinates as a point of projective space)
79
80
81
82 */
83
84
85 // points of type A
86
87 A1234:=[0,1,t,-tbar];
88 A4125:=[0,-1,t,-tbar];
89 A3152:=[0,1,-t,-tbar];
90 A5134:=[0,1,t,tbar];
91 A1253:=[0,-tbar,1,t];
92 A4153:=[0,tbar,1,t];
93 A3124:=[0,-tbar,-1,t];
94 A5142:=[0,-tbar,1,-t];
95 A1245:=[0,t,-tbar,1];
96 A4132:=[0,-t,-tbar,1];
97 A3145:=[0,t,tbar,1];
98 A5123:=[0,t,-tbar,-1];
99 A2345:=[0,1,0,0];
100 A2534:=[0,0,1,0];
101 A2435:=[0,0,0,1];
102
103 AA:=[
104 A1234,A4125,A3152,A5134,A1253,
105 A4153,A3124,A5142,A1245,A4132,
106 A3145,A5123,A2345,A2534,A2435
107 ];
108
109
110 // points of type B
111
112 B1234:=[2,1,t,-tbar];
113 B4125:=[2,-1,t,-tbar];
114 B3152:=[2,1,-t,-tbar];
115 B5134:=[2,1,t,tbar];
116
117 B2143:=[2,-1,-t,tbar];
118 B1452:=[2,1,-t,tbar];
119 B1325:=[2,-1,t,tbar];
120 B1543:=[2,-1,-t,-tbar];
121
122 B1253:=[2,-tbar,1,t];
123 B4153:=[2,tbar,1,t];
124 B3124:=[2,-tbar,-1,t];
125 B5142:=[2,-tbar,1,-t];
126
127 B2135:=[2,tbar,-1,-t];
128 B1435:=[2,-tbar,-1,-t];
129 B1342:=[2,tbar,1,-t];

```

```

130 B1524:=[2,tbar,-1,t];
131
132 B1245:=[2,t,-tbar,1];
133 B4132:=[2,-t,-tbar,1];
134 B3145:=[2,t,tbar,1];
135 B5123:=[2,t,-tbar,-1];
136
137 B2154:=[2,-t,tbar,-1];
138 B1423:=[2,t,tbar,-1];
139 B1354:=[2,-t,-tbar,-1];
140 B1532:=[2,-t,tbar,1];
141
142 B2345:=[1,1,0,0];
143 B3254:=[1,-1,0,0];
144 B2534:=[1,0,1,0];
145 B5243:=[1,0,-1,0];
146
147 B2453:=[1,0,0,1];
148 B4235:=[1,0,0,-1];
149
150
151 BB:=[
152 B1234,B4125,B3152,B5134,
153
154 B2143,B1452,B1325,B1543,
155
156 B1253,B4153,B3124,B5142,
157
158 B2135,B1435,B1342,B1524,
159
160 B1245,B4132,B3145,B5123,
161
162 B2154,B1423,B1354,B1532,
163
164 B2345,B3254,B2534,B5243,
165
166 B2453,B4235
167
168 ];
169
170 // points of type C
171
172 C12:=[1,1,1,1];
173 C41:=[1,-1,1,1];
174 C31:=[1,1,-1,1];
175 C51:=[1,1,1,-1];
176 C21:=[1,-1,-1,-1];
177 C14:=[1,1,-1,-1];
178 C13:=[1,-1,1,-1];
179 C15:=[1,-1,-1,1];
180 C53:=[1,0,-tbar,t];
181 C24:=[1,0,tbar,t];
182 C35:=[1,0,tbar,-t];
183 C42:=[1,0,-tbar,-t];
184 C45:=[1,t,0,-tbar];
185 C32:=[1,-t,0,-tbar];
186 C54:=[1,-t,0,tbar];
187 C23:=[1,t,0,tbar];
188 C34:=[1,-tbar,t,0];
189 C25:=[1,tbar,t,0];
190 C43:=[1,tbar,-t,0];

```

```

191 C52:=[1,-tbar,-t,0];
192
193 CC=[
194 C12, C41, C31, C51, C21,
195 C14, C13, C15, C53, C24,
196 C35, C42, C45, C32, C54,
197 C23, C34, C25, C43, C52
198 ];
199
200
201 // AA lines
202
203 listAA:={* *}; goodAA=[];
204
205 for i in [1..#AA] do
206     for j in [i+1..#AA] do
207
208         a1:=AA[i];
209         a2:=AA[j];
210         int:=intersect(a1,a2);
211         Include(~listAA, int);
212         if int eq {* 1^2, 2^2 *} then
213             Append(~goodAA, [i,j]);
214         end if;
215     end for;
216 end for;
217
218
219 /* summary:
220 60 A-A lines are contained in surface
221 (each passes through 5 nodes so actually only 6 lines)
222 30 A-A lines pass through 2 nodes plus another pt twice
223 (double check if the 3rd point is a node or a tangent -- probably node)
224 15 A-A lines pass through 2 nodes plus 2 distinct points
225 */
226
227
228 listAB:={* *}; goodAB=[];
229
230 for i in [1..#AA] do
231     for j in [1..#BB] do
232
233         a1:=AA[i];
234         a2:=BB[j];
235         int:=intersect(a1,a2);
236         Include(~listAB, int);
237         if int eq {* 1^2, 2^2 *} then
238             Append(~goodAB, [i,#AA+j]);
239         end if;
240     end for;
241 end for;
242
243 /*
244 60 A-B lines pass through 2 nodes plus 2 distinct points
245 390 A-B lines pass through 2 nodes plus another pt twice (check tangency?)
246 */
247
248
249 // AC lines
250
251 listAC:={* *}; goodAC=[];

```

```

252
253 for i in [1..#AA] do
254     for j in [1..#CC] do
255
256         a1:=AA[i];
257         a2:=CC[j];
258         int:=intersect(a1,a2);
259         Include(~listAC, int);
260         if int eq {* 1^2, 2^2 *} then
261             Append(~goodAC, [i,#AA+#BB+j]);
262         end if;
263     end for;
264 end for;
265
266 /*
267 A-C lines
268 60 A-C lines pass through 2 nodes plus 2 distinct points
269 240 A-C lines pass through 2 nodes plus another pt twice (check tangency?)
270 */
271
272
273 listBC:={* *}; goodBC:=[];
274
275 for i in [1..#BB] do
276     for j in [1..#CC] do
277
278         a1:=BB[i];
279         a2:=CC[j];
280         int:=intersect(a1,a2);
281         Include(~listBC, int);
282         if int eq {* 1^2, 2^2 *} then
283             Append(~goodBC, [#AA+i,#AA+#BB+j]);
284         end if; end for;
285 end for;
286
287 /*
288 120 B-C lines pass through 2 nodes plus 2 distinct points
289 240 B-C lines pass through 2 nodes (one with mult. 4)
290 240 B-C lines pass through 2 nodes plus another pt twice (check tangency?)
291 */
292
293
294 listBB:={* *}; goodBB:=[];
295
296 for i in [1..#BB] do
297     for j in [i+1..#BB] do
298
299         a1:=BB[i];
300         a2:=BB[j];
301         int:=intersect(a1,a2);
302         Include(~listBB, int);
303         if int eq {* 1^2, 2^2 *} then
304             Append(~goodBB, [#AA+i,#AA+j]);
305         end if;
306     end for;
307 end for;
308
309 /*
310 60 B-B lines pass through 2 nodes plus 2 distinct points
311 375 B-B lines pass through 2 nodes plus another pt twice (check tangency?)
312 */

```

```

313
314
315 listCC:={* *}; goodCC:=[];
316
317 for i in [1..#CC] do
318   for j in [i+1..#CC] do
319
320     a1:=CC[i];
321     a2:=CC[j];
322     int:=intersect(a1,a2);
323     Include(~listCC, int);
324     if int eq {* 1^2, 2^2 *} then
325       Append(~goodCC, [#AA+#BB+i, #AA+#BB+j]);
326     end if;
327   end for;
328 end for;
329
330
331 /* C-C lines
332 10 C-C lines pass through 2 nodes plus 2 distinct points
333 180 C-C lines pass through 2 nodes plus another point twice (check tangency)
334 */
335
336 good:=goodAA cat goodAB cat goodAC cat goodBB cat goodBC cat goodCC ;
337
338 GG:=Graph<65|{Set(x): x in good}>;
339 for v in VertexSet(GG) do #Sphere(v,1); end for; //10
340 for v in VertexSet(GG) do #Sphere(v,2); end for; //30
341 for v in VertexSet(GG) do #Sphere(v,3); end for; //24
342
343 IntersectionArray(GG); //[ 10, 6, 4, 1, 2, 5 ]
344
345 PG:=sub<GG|Neighbours(Vertices(GG)! 1)>; //check locally Petersen graph
346 for i in {1..65} do P2:=sub<GG|Neighbours(Vertices(GG)! i)>; IsIsomorphic(PG,P2);end for;//
    true

```

---

**4.2. Finding 2-planes in the Goryunov–Kalker cubic.** This script enumerates the 2-planes in the Goryunov–Kalker cubic 4-fold. It is used in *Part 2*, §2 in [2].

---

#### MAGMA 24. 2-planes in the Goryunov–Kalker cubic

---

```

1  /*
2  =====
3  2-Planes in Goryunov cubic
4  =====
5
6  Remarks:
7  =====
8  1. A posteriori, all planes are defined over the rationals so we do not
9  need any complicated field extensions.
10
11  2. It seems that all planes contained in chart 2 are already in chart 1
12  as well.
13

```

```

14 3. The planes are listed at the end of this file.
15
16 // First search for parametrised 2-planes contained in the cubic:
17
18 We consider the following two affine charts of Gr(3,7)
19
20 [ 1 0 0 a d g j ]
21 [ 0 1 0 b e h k ]
22 [ 0 0 1 c f i l ]
23
24 and
25
26 [ 1 0 a d g j 0 ]
27 [ 0 1 b e h k 0 ]
28 [ 0 0 c f i l 1 ]
29
30 Since the cubic has an action of S_6 permuting the x_i coordinates,
31 we can find all other 2-planes by calculating the orbits under S_6 of
32 planes contained in these two charts
33
34 */
35
36 // Set up parameters and variables
37
38 K<a,b,c,d,e,f,g,h,i,j,k,l>:=PolynomialRing(Rationals(),12);
39 R<u,v,w>:=PolynomialRing(K,3);
40
41 // chart 1
42
43 // parametrise 2-planes
44
45 List := [u,v,w,a*u+b*v+c*w,d*u+e*v+f*w,g*u+h*v+i*w,j*u+k*v+l*w];
46
47 // substitute into Goryunov cubic
48
49 x1:=List[1];
50 x2:=List[2];
51 x3:=List[3];
52 x4:=List[4];
53 x5:=List[5];
54 x6:=List[6];
55 x7:=List[7];
56
57 s1:=%+[x : x in [x1,x2,x3,x4,x5,x6]];
58 s3:=%+[x^3 : x in [x1,x2,x3,x4,x5,x6]];
59
60 // collect coefficients and find all points in parameter space
61 // where all coefficients vanish:
62
63 I := Coefficients(s1+2*x7) cat Coefficients(s3+2*x7^3);
64
65 // All points of the chart are rational, we do not need any field extension
66 // get 24 planes
67 Planes1:=Points(Scheme(Spec(K),I));
68 Planes1:=[Eltseq(p):p in Planes1];
69
70
71
72 // chart 2 -- same procedure, with different parametrisation
73
74 List := [u,v,a*u+b*v+c*w,d*u+e*v+f*w,g*u+h*v+i*w,j*u+k*v+l*w,w];

```

```

75
76 // substitute into Goryunov cubic
77
78
79 x1:=List[1];
80 x2:=List[2];
81 x3:=List[3];
82 x4:=List[4];
83 x5:=List[5];
84 x6:=List[6];
85 x7:=List[7];
86
87 s1:=%+[x : x in [x1,x2,x3,x4,x5,x6]];
88 s3:=%+[x^3 : x in [x1,x2,x3,x4,x5,x6]];
89
90 I := Coefficients(s1+2*x7) cat Coefficients(s3+2*x7^3);
91
92 // get 12 more planes
93 Planes2:=Points(Scheme(Spec(K),I));
94 Planes2:=[Eltseq(p):p in Planes2];
95
96 // now translate parametrised planes into embedded planes and
97
98 S<x1,x2,x3,x4,x5,x6,x7,u,v,w>:=PolynomialRing(Rationals(),7+3);
99
100 // chart 1:
101
102 // set containing all embedded planes
103 Planes:={};
104
105 for p in Planes1 do
106
107     Pi := [x1-u,x2-v,x3-w,
108           -x4+p[1]*u+p[2]*v+p[3]*w,
109           -x5+p[4]*u+p[5]*v+p[6]*w,
110           -x6+p[7]*u+p[8]*v+p[9]*w,
111           -x7+p[10]*u+p[11]*v+p[12]*w];
112     // convert to embedded plane
113
114     I:=Ideal(Pi);
115     J:=EliminationIdeal(I,{x1,x2,x3,x4,x5,x6,x7});
116
117     Include(~Planes,MinimalBasis(J));
118 end for;
119
120 // chart 2:
121
122 // include these planes in the original set of all planes because they
123 // are embedded now so the chart will no longer matter
124
125 for p in Planes2 do
126
127     Pi := [x1-u,x2-v,
128           -x3+p[1]*u+p[2]*v+p[3]*w,
129           -x4+p[4]*u+p[5]*v+p[6]*w,
130           -x5+p[7]*u+p[8]*v+p[9]*w,
131           -x6+p[10]*u+p[11]*v+p[12]*w,
132           x7-w];
133     // convert to embedded plane
134
135     I:=Ideal(Pi);

```



```

136     J:=EliminationIdeal(I,{x1,x2,x3,x4,x5,x6,x7});
137     Include(~Planes,MinimalBasis(J));
138 end for;
139
140
141 // now compute the S_6-orbits to find all planes in Goryunov cubic
142
143 // we set up an action of S_6 on the polynomial ring
144
145 PlaneOrbits:={};
146
147 G:=SymmetricGroup({x1,x2,x3,x4,x5,x6});
148 f:=Action(Orbit(G,x1));
149
150 // work out orbit of each plane found in charts 1 and 2:
151
152 for g in G do
153
154     // action of g as homomorphism on polynomial ring
155
156     phi:=hom<S->S|f(x1,g),f(x2,g),f(x3,g),f(x4,g),f(x5,g),f(x6,g),x7,u,v,w>;
157
158     for Pi in Planes do
159         Include(~PlaneOrbits,Ideal([phi(h):h in Pi]));
160     end for;
161
162 end for;
163
164
165 // can also compute the orbits individually.
166 // we find there are two orbits:
167
168 // partition of 6 in 2,2,2
169
170 x7 = x1 + x2 = x3 + x4 = x5 + x6 = 0 (15 planes)
171
172 and
173
174 // partition of 6 in 1,1,2,2
175
176 x1 + x2 = x3 + x4 = x5 + x7 = x6 + x7 = 0 (45 planes)
177
178 // we could have done this last step by hand, examining the list of planes found on the two
    charts, but its okay.

```

---

## REFERENCES

- [1] Fabrizio Catanese. Babbage's conjecture, contact of surfaces, symmetric determinantal varieties and applications. *Invent. Math.*, 63, no. 3, 433–465, (1981).
- [2] F. Catanese et al. Varieties of Nodal surfaces, coding theory and Discriminants of cubic hypersurfaces. preprint [arXiv:2206.05492](https://arxiv.org/abs/2206.05492), 2022.

INSTITUTE FOR BASIC SCIENCE - CENTER FOR COMPLEX GEOMETRY, 55 EXPO-RO YUSEONG-GU, DAEJEON  
34126, REPUBLIC OF KOREA

*Email address:* `yhcho88@ibs.re.kr`

MATHEMATISCHES INSTITUTE DER UNIVERSITÄT BAYREUTH, NW II, UNIVERSITÄTSSTR. 30, 95447 BAYREUTH,  
GERMANY

*Email address:* `Stephen.Coughlan@uni-bayreuth.de`

MATHEMATISCHES INSTITUTE DER UNIVERSITÄT BAYREUTH, NW II, UNIVERSITÄTSSTR. 30, 95447 BAYREUTH,  
GERMANY

*Email address:* `Davide.Frapporti@uni-bayreuth.de`

MATHEMATISCHES INSTITUTE DER UNIVERSITÄT BAYREUTH, NW II, UNIVERSITÄTSSTR. 30, 95447 BAYREUTH,  
GERMANY

*Email address:* `Kiermaier@uni-bayreuth.de`
